# Supplementary material for: Theoretical Prediction of the Effective Dynamic Dielectric Constant of Disordered Hyperuniform Anisotropic Composites Beyond the Long-Wavelength Regime
Source: arXiv:2312.05095 ancillary file (2023-12-22)
Supplement: Supplementary file 1 [file SM.pdf]

# Accurate Theoretical Prediction of the Effective Dynamic Dielectric Constant of Disordered Anisotropic Composites Beyond the Long-Wavelength Regime

## 1. GENERAL NONLOCAL STRONG-CONTRAST EXPANSION

### A. $n$ -Point Correlation Functions

A two-phase random medium is a domain of space partitioned into two disjoint regions: a phase 1 region  $\mathcal{V}_1$  of volume fraction  $\phi_1$  and a phase 2 region  $\mathcal{V}_2$  of volume fraction  $\phi_2$  [1]. The phase indicator function  $\mathcal{I}^{(i)}(\mathbf{x})$  of phase  $i$  for a given realization is defined as

$$\mathcal{I}^{(i)}(\mathbf{x}) = \begin{cases} 1, & \mathbf{x} \in \mathcal{V}_i, \\ 0, & \mathbf{x} \notin \mathcal{V}_i. \end{cases} \quad (\text{S1})$$

The  $n$ -point correlation function  $S_n^{(i)}$  for phase  $i$  is defined by [1, 2]:

$$S_n^{(i)}(\mathbf{x}_1, \dots, \mathbf{x}_n) = \left\langle \prod_{j=1}^n \mathcal{I}^{(i)}(\mathbf{x}_j) \right\rangle, \quad (\text{S2})$$

where angular brackets denote an ensemble average over realizations.

For statistically homogeneous media, the  $n$ -point correlation functions are translationally invariant. In particular,  $S_1^{(i)}(\mathbf{x}_1) = \phi_i$  and  $S_2^{(i)}(\mathbf{x}_1, \mathbf{x}_2) = S_2^{(i)}(\mathbf{r})$ , where  $\mathbf{r} \equiv \mathbf{x}_2 - \mathbf{x}_1$ . The function  $S_2^{(i)}(\mathbf{r})$  for phase  $i$  is simply related to the *autocovariance* function  $\chi_v(\mathbf{r}) \equiv S_2^{(i)}(\mathbf{r}) - \phi_i^2$ , which is independent of phase  $i$ . Thus,  $\chi_v(\mathbf{r} = 0) = \phi_1\phi_2$  and, assuming the medium possesses no long-range order,  $\lim_{|\mathbf{r}| \rightarrow \infty} \chi_v(\mathbf{r}) = 0$ . The nonnegative spectral density  $\tilde{\chi}_v(\mathbf{k})$  is the Fourier transform of  $\chi_v(\mathbf{r})$  at a wavevector  $\mathbf{k}$  and is proportional to scattering intensity [3] when  $\mathbf{k}$  is the momentum-transfer wavevector. For  $d$ -dimensional isotropic media, the spectral density depends only on  $k = |\mathbf{k}|$  and, its large- $k$  behavior is controlled by the following power-law form [1]:

$$\tilde{\chi}_v(k) \sim \frac{\gamma(d)s}{k^{d+1}}, \quad k \rightarrow \infty, \quad (\text{S3})$$

where  $\gamma(d) \equiv 2^{d-1}\pi^{d/2-1}\Gamma(d/2)$  is a  $d$ -dimensional constant,  $\Gamma(x)$  is the gamma function, and  $s$  is the specific surface (interface area per unit volume).

### B. Nonlocal Strong-Contrast Expansions in Three Dimensions

Here, we provide a brief review of the nonlocal strong-contrast expansions of the effective dynamic dielectric constant tensor  $\epsilon_e(\mathbf{k}_q, \omega)$  that treat statistically anisotropic two-phase composites in three dimensions, which was derived in Ref. [4]. We consider a macroscopically large two-phase composite specimen in three dimensions embedded inside an infinitely large reference phase  $q$  with the dielectric constant tensor  $\epsilon_q$ . The microstructure is perfectly general, and its characteristic inhomogeneity length scale  $\xi$  is much smaller than the specimen size  $L$ , i.e.,  $\xi \ll L$ . It is assumed that the applied or incident electric field  $\mathbf{E}_0(\mathbf{x})$  is a plane electric wave of an angular frequency  $\omega$  and a wavevector  $\mathbf{k}_q$  in the reference phase  $q$ . While one can take  $\epsilon_q$  to be any isotropic or anisotropic tensor that meets physical constraints, for the brevity of notation, we henceforth take the reference phase  $q$  as the matrix phase (i.e.,  $q = 1$  or  $2$ ) of the composite unless otherwise stated. For simplicity, we make three assumptions about both phases: (a) they have real-valued and frequency-independent dielectric constants, (b) they are dielectrically isotropic,

and (c) they are nonmagnetic. Due to these assumptions, the incident wavenumber  $k$  and frequency  $\omega$  are directly related by the linear dispersion relation, i.e.,  $k(\omega) \equiv |\mathbf{k}_q(\omega)| = \sqrt{\varepsilon_q} \omega / c$ , where  $c$  is the speed of light in vacuum. Thus, we henceforth do not explicitly indicate the  $\omega$  dependence, i.e.,  $\varepsilon_e(\mathbf{k}_q, \omega) = \varepsilon_e(\mathbf{k}_q)$

The strong-contrast expansions rely on the dyadic Green's function  $G^{(q)}(\mathbf{x} - \mathbf{x}')$  of the time-harmonic vector wave equation for the electric field in the reference phase  $q$  [4, 5]. Since  $G^{(q)}(\mathbf{x} - \mathbf{x}')$  has a singularity at  $\mathbf{x} = \mathbf{x}'$ , it is convenient to decompose  $G^{(q)}(\mathbf{x} - \mathbf{x}')$  into two terms:

$$G^{(q)}(\mathbf{r}) = -D^{(q)} \delta(\mathbf{r}) + H^{(q)}(\mathbf{r}), \quad (\text{S4})$$

where a constant second-rank tensor  $D^{(q)}$ , called the source dyadic [4, 6], arises from an infinitesimal region around the position of the singularity  $\mathbf{x}' = \mathbf{x}$  in the Green's function, and  $H^{(q)}(\mathbf{r})$  represents the contribution exterior to the singularity. For an isotropic reference phase in three dimensions, the principal part of the Green's function (outside the exclusion volume) is

$$H^{(q)}(\mathbf{r}) = \frac{\exp(ikr)}{\varepsilon_q 4\pi r^3} [-1 + ikr + (kr)^2] \mathbf{I} + \frac{\exp(ikr)}{\varepsilon_q 4\pi r^3} [3 - 3ikr - (kr)^2] \hat{\mathbf{r}}\hat{\mathbf{r}}, \quad (\text{S5})$$

where  $\hat{\mathbf{r}} \equiv \mathbf{r}/|\mathbf{r}|$  is a unit vector. The formula [Eq. (S4)] together with Eq. (S5) is the temporal Fourier transform of the retarded Green's function that accounts for the causality.

The nonlocal strong-contrast expansion is a series expansion of the effective tensor  $[L_e(\mathbf{k}_q)]^{-1}$ , a linear fractional form of the effective dynamic dielectric constant  $\varepsilon_e(\mathbf{k}_q)$ , and can be written as

$$\phi_p L_p^{(q)} \cdot [L_e(\mathbf{k}_q)]^{-1} \cdot \phi_p L_p^{(q)} = \phi_p L_p^{(q)} - \sum_{n=2}^{\infty} \mathcal{A}_n^{(p)}(\mathbf{k}_q), \quad (\text{S6})$$

where

$$L_p^{(q)} \equiv (\varepsilon_p - \varepsilon_q) [\mathbf{I} + D^{(q)}(\varepsilon_p - \varepsilon_q)]^{-1}, \quad (\text{S7})$$

$$L_e^{(q)}(\mathbf{k}_q) \equiv [\varepsilon_e(\mathbf{k}_q) - \varepsilon_q \mathbf{I}] \cdot \{\mathbf{I} + D^{(q)} \cdot [\varepsilon_e(\mathbf{k}_q) - \varepsilon_q \mathbf{I}]\}^{-1}, \quad (\text{S8})$$

and  $\mathcal{A}_n^{(p)}(\mathbf{k}_q)$  is a wavevector-dependent second-rank tensor that is a functional involving the set of correlation functions  $S_1^{(p)}, S_2^{(p)}, \dots, S_n^{(p)}$  and products of the principal part of the dyadic Green's function  $H^{(q)}(\mathbf{r})$ . Specifically,

$$\mathcal{A}_2^{(p)}(\mathbf{k}_q) \equiv L_p^{(q)} \cdot \left[ \int_{\epsilon} d\mathbf{x}_1 H^{(q)}(\mathbf{x}_1 - \mathbf{x}_2) e^{-i\mathbf{k}_q \cdot (\mathbf{x}_1 - \mathbf{x}_2)} \chi_V(\mathbf{x}_1 - \mathbf{x}_2) \right] \cdot L_p^{(q)}, \quad (\text{S9})$$

$$\begin{aligned} \mathcal{A}_n^{(p)}(\mathbf{k}_q) \equiv & \left( \frac{-1}{\phi_p} \right)^{n-2} \int_{\epsilon} d\mathbf{x}_1 \cdots d\mathbf{x}_{n-1} \prod_{j=1}^{n-1} \left[ L_p^{(q)} \cdot H^{(q)}(\mathbf{x}_j - \mathbf{x}_{j+1}) e^{-i\mathbf{k}_q \cdot (\mathbf{x}_j - \mathbf{x}_{j+1})} \right] \\ & \cdot L_p^{(q)} \Delta_n^{(p)}(\mathbf{x}_1, \dots, \mathbf{x}_n), \quad (n > 2), \end{aligned} \quad (\text{S10})$$

where  $\int_{\epsilon} d\mathbf{r}$  stands for the Cauchy principal value of the integral by omitting the exclusion volume around the origin, and  $\Delta_n^{(p)}$  is a position-dependent determinant involving  $m$ -point correlation function  $S_m^{(p)}$  of the polarized phase  $p$  up to the  $n$ -point level:

$$\Delta_n^{(p)}(\mathbf{x}_1, \dots, \mathbf{x}_n) = \begin{vmatrix} S_2^{(p)}(\mathbf{x}_1, \mathbf{x}_2) & S_1^{(p)}(\mathbf{x}_1) & \cdots & 0 \\ S_3^{(p)}(\mathbf{x}_1, \mathbf{x}_2, \mathbf{x}_3) & S_2^{(p)}(\mathbf{x}_2, \mathbf{x}_3) & \cdots & 0 \\ \vdots & \vdots & \ddots & \vdots \\ S_n^{(p)}(\mathbf{x}_1, \dots, \mathbf{x}_n) & S_{n-1}^{(p)}(\mathbf{x}_2, \dots, \mathbf{x}_n) & \cdots & S_2^{(p)}(\mathbf{x}_{n-1}, \mathbf{x}_n) \end{vmatrix}. \quad (\text{S11})$$

The strong-contrast expansion (S6) has four important features:

1. This expansion is established based on a spatially nonlocal constitutive relation, i.e., the average polarization field at position  $\mathbf{x}$  depends on the average electric field at other positions around  $\mathbf{x}$  [7–10], which is valid from the long- to intermediate-wavelength regimes, i.e.,  $0 \leq |\mathbf{k}_q| \xi \lesssim 1$ , where  $\xi$  is a characteristic inhomogeneity length scale. Specifically, the

51 exact strong-contrast expansion (S6) relies on the following *nonlocal* constitutive relation  
 52 relates ensemble averages of the polarization vector  $\mathbf{P}(\mathbf{x})$  and the *cavity intensity field*  $\mathbf{F}(\mathbf{x})$   
 53 [4]:

$$\langle \mathbf{P} \rangle(\mathbf{x}) = \int d\mathbf{x}' L_e^{(q)}(\mathbf{x} - \mathbf{x}') \cdot \langle \mathbf{F} \rangle(\mathbf{x}'), \quad (\text{S12})$$

which is reduced to a linear product by taking the Fourier transform as follows:

$$\widetilde{\langle \mathbf{P} \rangle}(\mathbf{k}_q) = L_e^{(q)}(\mathbf{k}_q) \cdot \widetilde{\langle \mathbf{F} \rangle}(\mathbf{k}_q). \quad (\text{S13})$$

This relation is equivalent to the popular nonlocal constitutive relation [4]:

$$\widetilde{\langle \mathbf{D} \rangle}(\mathbf{k}) = \varepsilon_0 \varepsilon_e(\mathbf{k}) \cdot \widetilde{\langle \mathbf{E} \rangle}(\mathbf{k}), \quad (\text{S14})$$

54 where  $\varepsilon_0$  is the dielectric permittivity of vacuum.

- 55 2. The representation (S6) exactly treats multiple scattering to all orders at a given inci-  
 56 dent wavevector  $\mathbf{k}_q$  when the nonlocal homogenization theory is valid because the terms  
 57  $\mathcal{A}_n^{(p)}(\mathbf{k}_q)$  for  $n = 2, \dots$  in this series explicitly account for complete microstructural infor-  
 58 mation (the infinite set of  $S_2, S_3, \dots$ ) to infinite order.
- 59 3. A choice for the shape of the infinitesimal exclusion volume determines symmetries of  
 60 a tensor  $\mathbf{D}^{(q)}$ . We present some important examples for an isotropic reference phase  $q$  as  
 61 follows [4, 6]:

$$\mathbf{D}^{(q)} = \begin{cases} \frac{1}{3\varepsilon_q} \mathbf{I}, & \text{spherical exclusion volume} \\ \frac{1}{\varepsilon_q} \hat{\mathbf{z}}\hat{\mathbf{z}}, & \text{disk-like exclusion volume perpendicular to the } z \text{ axis,} \\ \frac{1}{2\varepsilon_q} (\mathbf{I} - \hat{\mathbf{z}}\hat{\mathbf{z}}), & \text{needle-like exclusion volume aligned with the } z \text{ axis} \end{cases} \quad (\text{S15})$$

62 where its trace  $\text{Tr}[\mathbf{D}^{(q)}]$  is always independent of the exclusion volume shape [6]:  $\text{Tr}[\mathbf{D}^{(q)}] \equiv$   
 63  $\mathbf{I} : \mathbf{D}^{(q)} = 1/\varepsilon_q$ . Thus, a different choice of the exclusion-region shape leads to a different  
 64 expansion parameter  $L_p^{(q)}$  and expansion with significantly different convergence properties.  
 65 For this reason, different from the standard multiple-scattering theory [11–14], one can  
 66 naturally ‘tune’ the general series expansions to obtain distinctly different approximations  
 67 suited for certain classes of microstructures.

- 68 4. The left-handed side of the series [Eq. (S6)] is a linear fractional transformation of  $\varepsilon_e(\mathbf{k}_q)$   
 69 rather than  $\varepsilon_e(\mathbf{k}_q)$  itself, which leads to the rapid convergence of the strong-contrast expan-  
 70 sions in that the lower-order truncations of the series can well approximate higher-order  
 71 functionals (i.e., higher-order diagrams) of the exact series to all orders in terms of lower-  
 72 order diagrams; see Sec. IIIB of Ref. [4] for details.

Features 1, 3, and 4 are particularly important to extract accurate multiple-scattering approxi-  
 mations from the exact series [Eq. (S6)]. Feature 1 extends the validity range in which Eq. (S6)  
 through the infinite order can provide an exact estimation of  $\varepsilon_e(\mathbf{k}_q, \omega)$ . Within such an extended  
 validity range, however, it is increasingly challenging to compute the higher-order terms  $\mathcal{A}_n^{(p)}(\mathbf{k}_q)$   
 for  $n > 2$ . Thus, in practice, it is useful to consider the  $n$ th-order truncations of Eq. (S6) as accurate  
 multiple-scattering approximations, i.e.,

$$\phi_p L_p^{(q)} \cdot [L_e(\mathbf{k}_q)]^{-1} \cdot \phi_p L_p^{(q)} = \phi_p L_p^{(q)} - \mathcal{A}_2^{(p)}(\mathbf{k}_q) - \mathcal{A}_3^{(p)}(\mathbf{k}_q) - \dots - \mathcal{A}_n^{(p)}(\mathbf{k}_q). \quad (\text{S16})$$

73 Due to Features 3 and 4, when expansion parameter  $L_p^{(q)}$  and the reference phase  $\varepsilon_q$  are judiciously  
 74 chosen, even the second- or third-order truncations can lead to approximations that can be  
 75 very accurate for a wide range of contrast ratios and classes of microstructures with various  
 76 symmetries.

### 77 C. Fourier Representations of the Strong-Contrast Expansions

78 Here, we provide the Fourier representation of the coefficients  $\mathcal{A}_n^{(p)}(\mathbf{k}_q)$  given in Eq. (S9) and  
 79 Eq. (S10). Throughout this work, we mainly use these Fourier representations because the Fourier  
 80 transform of the dyadic Green's function given in Eq. (S4) is particularly simple and concise<sup>1</sup>:

$$\tilde{G}_{ij}^{(q)}(\mathbf{k}) = \frac{1}{\varepsilon_q} \frac{k_q^2 \delta_{ij} - k_i k_j}{k^2 - k_q^2}. \quad (\text{S17})$$

Note that Eq. (S17) is independent of the shape of the exclusion volume, which stands in contrast to the shape-dependent Fourier transform of  $H_{ij}^{(q)}(\mathbf{r})$ :

$$\tilde{H}^{(q)}(\mathbf{k}) = \tilde{G}^{(q)}(\mathbf{k}) + \mathbf{D}^{(q)} = \frac{1}{\varepsilon_q} \frac{k_q^2 \mathbf{I} - \mathbf{k}\mathbf{k}}{k^2 - k_q^2} + \mathbf{D}^{(q)}. \quad (\text{S18})$$

Here, we present the Fourier representations of the first three coefficients  $\mathcal{A}_2^{(p)}(\mathbf{k}_q)$ ,  $\mathcal{A}_3^{(p)}(\mathbf{k}_q)$ , and  $\mathcal{A}_4^{(p)}(\mathbf{k}_q)$  given in Eq. (S9) and Eq. (S10):

$$\begin{aligned} \mathcal{A}_2^{(p)}(\mathbf{k}_q) &= \frac{1}{(2\pi)^3} \int d\mathbf{q} \left[ \mathbf{L}_p^{(q)} \cdot \tilde{H}^{(q)}(\mathbf{k}_q + \mathbf{q}) \right] \cdot \mathbf{L}_p^{(q)} \tilde{\chi}_v(\mathbf{q}) \\ &= \mathbf{L}_p^{(q)} \cdot \left\{ \frac{1}{(2\pi)^3} \int d\mathbf{q} \left[ \frac{1}{\varepsilon_q} \frac{k^2 \mathbf{I} - (\mathbf{q} + \mathbf{k}_q)(\mathbf{q} + \mathbf{k}_q)}{|\mathbf{q} + \mathbf{k}_q|^2 - k^2} + \mathbf{D}^{(q)} \right] \tilde{\chi}_v(\mathbf{q}) \right\} \cdot \mathbf{L}_p^{(q)}, \end{aligned} \quad (\text{S19})$$

$$\mathcal{A}_3^{(p)}(\mathbf{k}_q) = \left( \frac{-1}{\phi_p} \right) \frac{1}{(2\pi)^{2 \cdot 3}} \int d\mathbf{q}_1 d\mathbf{q}_2 \left[ \mathbf{L}_p^{(q)} \cdot \tilde{H}^{(q)}(\mathbf{k}_q + \mathbf{q}_1) \cdot \mathbf{L}_p^{(q)} \cdot \tilde{H}^{(q)}(\mathbf{k}_q + \mathbf{q}_2) \right] \cdot \mathbf{L}_p^{(q)} \tilde{\Delta}_3^{(p)}(\mathbf{q}_1, \mathbf{q}_2), \quad (\text{S20})$$

$$\begin{aligned} \mathcal{A}_4^{(p)}(\mathbf{k}_q) &= \left( \frac{-1}{\phi_p} \right)^2 \frac{1}{(2\pi)^{3 \cdot 3}} \int d\mathbf{q}_1 d\mathbf{q}_2 d\mathbf{q}_3 \left[ \mathbf{L}_p^{(q)} \cdot \tilde{H}^{(q)}(\mathbf{k}_q + \mathbf{q}_1) \cdot \mathbf{L}_p^{(q)} \cdot \tilde{H}^{(q)}(\mathbf{k}_q + \mathbf{q}_2) \cdot \mathbf{L}_p^{(q)} \cdot \tilde{H}^{(q)}(\mathbf{k}_q + \mathbf{q}_3) \right] \\ &\quad \cdot \mathbf{L}_p^{(q)} \tilde{\Delta}_4^{(p)}(\mathbf{q}_1, \mathbf{q}_2, \mathbf{q}_3), \end{aligned} \quad (\text{S21})$$

81 where we have used the convolution theorem, and  $\tilde{\Delta}_n^{(p)}(\mathbf{q}_1, \dots, \mathbf{q}_{n-1})$  is the Fourier transform of  
 82 Eq. (S11) for  $n \geq 3$ .

To derive expressions for  $\tilde{\Delta}_n^{(p)}(\mathbf{q}_1, \dots, \mathbf{q}_{n-1})$ , we rewrite Eq. (S11) for  $n = 3, 4$  in terms of the fluctuating part of the phase indicator function

$$\mathcal{J}^{(p)}(\mathbf{x}) \equiv \mathcal{I}^{(p)}(\mathbf{x}) - \phi_p, \quad (\text{S22})$$

as follows:

$$\Delta_3^{(p)}(\mathbf{x}_1, \mathbf{x}_2, \mathbf{x}_3) = \chi_v(\mathbf{x}_1, \mathbf{x}_2) \chi_v(\mathbf{x}_2, \mathbf{x}_3) - \phi_p \langle \mathcal{J}^{(p)}(\mathbf{x}_1) \mathcal{J}^{(p)}(\mathbf{x}_2) \mathcal{J}^{(p)}(\mathbf{x}_3) \rangle - \phi_p^2 \chi_v(\mathbf{x}_1, \mathbf{x}_3), \quad (\text{S23})$$

$$\begin{aligned} \Delta_4^{(p)}(\mathbf{x}_1, \dots, \mathbf{x}_4) &\equiv \phi_p^2 S_4^{(p)}(\mathbf{x}_1, \dots, \mathbf{x}_4) + S_2^{(p)}(\mathbf{x}_1, \mathbf{x}_2) S_2^{(p)}(\mathbf{x}_2, \mathbf{x}_3) S_2^{(p)}(\mathbf{x}_3, \mathbf{x}_4) \\ &\quad - \phi_p S_2^{(p)}(\mathbf{x}_1, \mathbf{x}_2) S_3^{(p)}(\mathbf{x}_2, \mathbf{x}_3, \mathbf{x}_4) - \phi_p S_2^{(p)}(\mathbf{x}_3, \mathbf{x}_4) S_3^{(p)}(\mathbf{x}_1, \mathbf{x}_2, \mathbf{x}_3) \\ &= \phi_p^2 S_4^{(p)}(\mathbf{x}_1, \dots, \mathbf{x}_4) - S_2^{(p)}(\mathbf{x}_1, \mathbf{x}_2) S_2^{(p)}(\mathbf{x}_2, \mathbf{x}_3) S_2^{(p)}(\mathbf{x}_3, \mathbf{x}_4) \\ &\quad + S_2^{(p)}(\mathbf{x}_1, \mathbf{x}_2) \Delta_3^{(p)}(\mathbf{x}_2, \mathbf{x}_3, \mathbf{x}_4) + S_2^{(p)}(\mathbf{x}_3, \mathbf{x}_4) \Delta_3^{(p)}(\mathbf{x}_1, \mathbf{x}_2, \mathbf{x}_3) \\ &= \phi_p^4 \chi_v(\mathbf{x}_1, \mathbf{x}_4) + \phi_p^3 \left[ \langle \mathcal{J}^{(p)}(\mathbf{x}_1) \mathcal{J}^{(p)}(\mathbf{x}_2) \mathcal{J}^{(p)}(\mathbf{x}_4) \rangle + \langle \mathcal{J}^{(p)}(\mathbf{x}_1) \mathcal{J}^{(p)}(\mathbf{x}_3) \mathcal{J}^{(p)}(\mathbf{x}_4) \rangle \right] \\ &\quad + \phi_p^2 \left[ \langle \mathcal{J}^{(p)}(\mathbf{x}_1) \mathcal{J}^{(p)}(\mathbf{x}_2) \mathcal{J}^{(p)}(\mathbf{x}_3) \mathcal{J}^{(p)}(\mathbf{x}_4) \rangle - \chi_v(\mathbf{x}_1, \mathbf{x}_2) \chi_v(\mathbf{x}_3, \mathbf{x}_4) \right] \\ &\quad - \chi_v(\mathbf{x}_1, \mathbf{x}_2) \chi_v(\mathbf{x}_2, \mathbf{x}_3) \chi_v(\mathbf{x}_3, \mathbf{x}_4) + \chi_v(\mathbf{x}_1, \mathbf{x}_2) \Delta_3^{(p)}(\mathbf{x}_2, \mathbf{x}_3, \mathbf{x}_4) + \chi_v(\mathbf{x}_3, \mathbf{x}_4) \Delta_3^{(p)}(\mathbf{x}_1, \mathbf{x}_2, \mathbf{x}_3), \end{aligned} \quad (\text{S24})$$

<sup>1</sup>General expressions for  $\tilde{H}^{(q)}(\mathbf{k})$  and  $\mathbf{D}^{(q)}$  in an anisotropic reference phase with  $\varepsilon_q$  are discussed in Ref. [8].

where  $\chi_v(\mathbf{x}_1, \mathbf{x}_2) \equiv \langle \mathcal{J}^{(p)}(\mathbf{x}_1) \mathcal{J}^{(p)}(\mathbf{x}_2) \rangle$ . Then,  $\tilde{\Delta}_3^{(p)}$  and  $\tilde{\Delta}_4^{(p)}$  from Eq. (S23) and Eq. (S24) are written explicitly as follows:

$$\begin{aligned} \tilde{\Delta}_3^{(p)}(\mathbf{q}_1, \mathbf{q}_2) &\equiv \int d\mathbf{r} d\mathbf{s} e^{-i\mathbf{q}_1 \cdot \mathbf{r}} e^{-i\mathbf{q}_2 \cdot \mathbf{s}} \Delta_3^{(p)}(\mathbf{x}_1, \mathbf{x}_2, \mathbf{x}_3) \\ &= -\phi_p \int d\mathbf{r} d\mathbf{s} e^{-i\mathbf{q}_1 \cdot \mathbf{x}_1} e^{-i(\mathbf{q}_2 - \mathbf{q}_1) \cdot (\mathbf{x}_1 - \mathbf{r})} e^{-i(-\mathbf{q}_2) \cdot (\mathbf{x}_1 - \mathbf{r} - \mathbf{s})} \langle \mathcal{J}^{(p)}(\mathbf{x}_1) \mathcal{J}^{(p)}(\mathbf{x}_1 - \mathbf{r}) \mathcal{J}^{(p)}(\mathbf{x}_1 - \mathbf{r} - \mathbf{s}) \rangle \\ &\quad - \phi_p^2 \int d\mathbf{r} d\mathbf{s} [e^{-i(\mathbf{q}_1 - \mathbf{q}_2) \cdot \mathbf{r}} e^{-i\mathbf{q}_2 \cdot (\mathbf{r} + \mathbf{s})} \chi_v(\mathbf{r} + \mathbf{s})] + \tilde{\chi}_v(\mathbf{q}_1) \tilde{\chi}_v(\mathbf{q}_2) \\ &= -\phi_p \langle \tilde{\mathcal{J}}^{(p)}(\mathbf{q}_1) \tilde{\mathcal{J}}^{(p)}(\mathbf{q}_2 - \mathbf{q}_1) \tilde{\mathcal{J}}^{(p)}(-\mathbf{q}_2) \rangle \\ &\quad - \phi_p^2 (2\pi)^3 \delta(\mathbf{q}_1 - \mathbf{q}_2) \tilde{\chi}_v(\mathbf{q}_2) + \tilde{\chi}_v(\mathbf{q}_1) \tilde{\chi}_v(\mathbf{q}_2), \end{aligned} \quad (\text{S25})$$

$$\begin{aligned} \tilde{\Delta}_4^{(p)}(\mathbf{q}_1, \mathbf{q}_2, \mathbf{q}_3) &\equiv \int d\mathbf{r} d\mathbf{s} d\mathbf{t} e^{-i\mathbf{q}_1 \cdot \mathbf{r}} e^{-i\mathbf{q}_2 \cdot \mathbf{s}} e^{-i\mathbf{q}_3 \cdot \mathbf{t}} \Delta_4^{(p)}(\mathbf{x}_1, \dots, \mathbf{x}_4) \\ &= \phi_p^4 (2\pi)^6 \delta(\mathbf{q}_2 - \mathbf{q}_3) \delta(\mathbf{q}_1 - \mathbf{q}_3) \tilde{\chi}_v(\mathbf{q}_3) \\ &\quad + \phi_p^3 (2\pi)^3 [\langle \tilde{\mathcal{J}}^{(p)}(\mathbf{q}_1) \tilde{\mathcal{J}}^{(p)}(-\mathbf{q}_1 + \mathbf{q}_2) \tilde{\mathcal{J}}^{(p)}(-\mathbf{q}_3) \rangle \delta(\mathbf{q}_3 - \mathbf{q}_2) \\ &\quad + \langle \tilde{\mathcal{J}}^{(p)}(\mathbf{q}_1) \tilde{\mathcal{J}}^{(p)}(-\mathbf{q}_2 + \mathbf{q}_3) \tilde{\mathcal{J}}^{(p)}(-\mathbf{q}_3) \rangle \delta(\mathbf{q}_2 - \mathbf{q}_1)] \\ &\quad + \phi_p^2 [\langle \tilde{\mathcal{J}}^{(p)}(\mathbf{q}_1) \tilde{\mathcal{J}}^{(p)}(-\mathbf{q}_1 + \mathbf{q}_2) \tilde{\mathcal{J}}^{(p)}(-\mathbf{q}_2 + \mathbf{q}_3) \tilde{\mathcal{J}}^{(p)}(-\mathbf{q}_3) \rangle - (2\pi)^3 \delta(\mathbf{q}_2) \tilde{\chi}_v(\mathbf{q}_1) \tilde{\chi}_v(\mathbf{q}_3)] \\ &\quad - \tilde{\chi}_v(\mathbf{q}_1) \tilde{\chi}_v(\mathbf{q}_2) \tilde{\chi}_v(\mathbf{q}_3) + \tilde{\chi}_v(\mathbf{q}_1) \tilde{\Delta}_3^{(p)}(\mathbf{q}_2, \mathbf{q}_3) + \tilde{\chi}_v(\mathbf{q}_3) \tilde{\Delta}_3^{(p)}(\mathbf{q}_1, \mathbf{q}_2) \quad (\text{S26}) \\ &= -\phi_p^4 (2\pi)^6 \delta(\mathbf{q}_1 - \mathbf{q}_2) \delta(\mathbf{q}_2 - \mathbf{q}_3) \tilde{\chi}_v(\mathbf{q}_2) + \phi_p^2 (2\pi)^3 [\delta(\mathbf{q}_3 - \mathbf{q}_2) + \delta(\mathbf{q}_1 - \mathbf{q}_2) - \delta(\mathbf{q}_2)] \tilde{\chi}_v(\mathbf{q}_1) \tilde{\chi}_v(\mathbf{q}_3) \\ &\quad + \phi_p^2 \langle \tilde{\mathcal{J}}^{(p)}(\mathbf{q}_1) \tilde{\mathcal{J}}^{(p)}(-\mathbf{q}_1 + \mathbf{q}_2) \tilde{\mathcal{J}}^{(p)}(-\mathbf{q}_2 + \mathbf{q}_3) \tilde{\mathcal{J}}^{(p)}(-\mathbf{q}_3) \rangle - \tilde{\chi}_v(\mathbf{q}_1) \tilde{\chi}_v(\mathbf{q}_2) \tilde{\chi}_v(\mathbf{q}_3) \\ &\quad + [\tilde{\chi}_v(\mathbf{q}_1) - \phi_p^2 (2\pi)^3 \delta(\mathbf{q}_1 - \mathbf{q}_2)] \tilde{\Delta}_3^{(p)}(\mathbf{q}_2, \mathbf{q}_3) + [\tilde{\chi}_v(\mathbf{q}_3) - \phi_p^2 (2\pi)^3 \delta(\mathbf{q}_3 - \mathbf{q}_2)] \tilde{\Delta}_3^{(p)}(\mathbf{q}_1, \mathbf{q}_2), \end{aligned} \quad (\text{S27})$$

where  $\mathbf{r} \equiv \mathbf{x}_1 - \mathbf{x}_2$ ,  $\mathbf{s} \equiv \mathbf{x}_2 - \mathbf{x}_3$ ,  $\mathbf{t} \equiv \mathbf{x}_3 - \mathbf{x}_4$ , and  $\tilde{\mathcal{J}}^{(p)}(\mathbf{q})$  is the Fourier transform of Eq. (S22).

## 2. NONLOCAL STRONG-CONTRAST EXPANSIONS FOR LAYERED MEDIA

Here, we present a detailed derivation of our multiple-scattering approximations of  $\varepsilon_e(\mathbf{k}_q)$  for 3D two-phase layered media. This section includes some details that we omitted in a derivation for the normal incidence case in Ref. [15]. We begin by describing how to utilize the symmetries of layered media in the general expansions. We then truncate the resulting expansion at the  $n$ -point level for extracting multiple-scattering approximations of  $\varepsilon_e(\mathbf{k}_q)$  suited for layered media.

### A. Symmetries of Layered Media

Layered media have rotational symmetry around the  $z$ -axis and translational symmetry along the  $x$ - $y$  plane; see Fig. 1(a) of the main text. Due to the symmetries, the  $n$ -point correlation function depends solely on the  $z$  coordinates of relative positions and thus can be reduced to that in one dimension:  $S_n^{(i)}(\mathbf{x}_1, \dots, \mathbf{x}_n) = S_n^{(i)}(z_2 - z_1, \dots, z_n - z_1)$ . Consequently, the corresponding spectral density or the Fourier transform of  $\Delta_n^{(p)}(\mathbf{x}_1, \dots, \mathbf{x}_n)$  given in Eq. (S11) can be simplified, respectively, as follows:

$$\tilde{\chi}_v(\mathbf{q}) = (2\pi)^2 \delta([\mathbf{q}]_{\perp}) \tilde{\chi}_v(q_z), \quad (\text{S28})$$

$$\tilde{\Delta}_n^{(p)}(\mathbf{q}_1, \dots, \mathbf{q}_{n-1}) = (2\pi)^{2(n-1)} \delta([\mathbf{q}_1]_{\perp}) \dots \delta([\mathbf{q}_{n-1}]_{\perp}) \tilde{\Delta}_n^{(p)}(q_{1z}, \dots, q_{n-1z}), \quad n = 3, \dots, \quad (\text{S29})$$

where  $\delta([\mathbf{q}]_{\perp})$  is the two-dimensional Dirac delta function, and  $\tilde{\chi}_v(q_z)$  is the spectral density of the 1D media, from which the layered media are derived. To utilize the symmetries of layered media, we choose a disk-like exclusion volume normal to the symmetry axis (i.e.,  $z$ -axis), leading to

$$\mathbf{D}^{(q)} = \frac{1}{\varepsilon_q} \hat{\mathbf{z}} \hat{\mathbf{z}}, \quad (\text{S30})$$

$$\mathbf{L}_p^{(q)} = \beta_{pq}^{(1D)} [\varepsilon_p (\mathbf{I} - \hat{\mathbf{z}} \hat{\mathbf{z}}) + \varepsilon_q \hat{\mathbf{z}} \hat{\mathbf{z}}], \quad (\text{S31})$$

where we have obtained the expansion parameter [Eq. (S31)] by substituting Eq. (S30) into Eq. (S7),  $\hat{\mathbf{z}}$  is a unit vector along the z-direction, and  $\beta_{pq}^{(1D)} \equiv 1 - \varepsilon_q/\varepsilon_p$  is the one-dimensional counterpart of the *dielectric polarizability*. Then, using Eq. (S30) and Eq. (S31), we rewrite Eq. (S18) as

$$\tilde{\mathbf{H}}^{(q)}(\mathbf{k}) = \frac{1}{\varepsilon_q} \left( \frac{k_q^2 \mathbf{I} - \mathbf{k}\mathbf{k}}{k^2 - k_q^2} + \hat{\mathbf{z}}\hat{\mathbf{z}} \right) = \frac{1}{\varepsilon_q} \frac{k_q^2 (\mathbf{I} - \hat{\mathbf{z}}\hat{\mathbf{z}}) + k^2 \hat{\mathbf{z}}\hat{\mathbf{z}} - \mathbf{k}\mathbf{k}}{k^2 - k_q^2} \quad (\text{S32})$$

## 91 B. Multiple-Scattering Approximations: General Cases

92 We begin from the multiple-scattering approximation given in Eq. (S16). Therein, we derive  
 93 explicit expressions for the first two coefficients  $\mathcal{A}_n^{(p)}(\mathbf{k}_q)$  for  $n = 2, 3$  in layered media by  
 94 substituting Eq. (S30) and Eq. (S31) into it. Without losing generality, we assume an obliquely  
 95 incident wavevector  $\mathbf{k}_q = k_q(\hat{\mathbf{z}} \cos \theta + \hat{\mathbf{x}} \sin \theta)$ , where  $\theta$  is the incidence angle.

We first derive the explicit expression of  $\mathcal{A}_2^{(p)}(\mathbf{k}_q)$  for stratified media. After a brief algebra, from Eq. (S31) and Eq. (S32), we obtain

$$\begin{aligned} L_p^{(q)} \cdot \tilde{\mathbf{H}}^{(q)}(\mathbf{k}) \cdot L_p^{(q)} &= \frac{1}{\varepsilon_q} \frac{\beta_{pq}^2}{k^2 - k_q^2} \left( \varepsilon_p^2 \{k_q^2 (\mathbf{I} - \hat{\mathbf{z}}\hat{\mathbf{z}}) - [\mathbf{k}]_{\perp} [\mathbf{k}]_{\perp}\} - \varepsilon_q \varepsilon_p k_z (\hat{\mathbf{z}} [\mathbf{k}]_{\perp} + [\mathbf{k}]_{\perp} \hat{\mathbf{z}}) \right. \\ &\quad \left. + \varepsilon_q^2 (k_q^2 - k_z^2) \hat{\mathbf{z}}\hat{\mathbf{z}} \right) + \varepsilon_q \beta_{pq}^2 \hat{\mathbf{z}}\hat{\mathbf{z}}, \end{aligned} \quad (\text{S33})$$

where for a vector  $\mathbf{k}$ ,  $k_z \equiv \mathbf{k} \cdot \hat{\mathbf{z}}$  and  $[\mathbf{k}]_{\perp} \equiv \mathbf{k} \cdot (\mathbf{I} - \hat{\mathbf{z}}\hat{\mathbf{z}}) = k_x \hat{\mathbf{x}} + k_y \hat{\mathbf{y}}$ . Expression for  $\mathcal{A}_2^{(p)}(\mathbf{k})$  is obtained by substituting Eq. (S28) and Eq. (S33) into Eq. (S19):

$$\begin{aligned} \mathcal{A}_2^{(p)}(\mathbf{k}_q) &= \frac{1}{(2\pi)^3} \int d\mathbf{q} L_p^{(q)} \cdot \tilde{\mathbf{H}}^{(q)}(\mathbf{k}_q + \mathbf{q}) \cdot L_p^{(q)} \tilde{\chi}_v(\mathbf{q}) \\ &= \frac{1}{2\pi} \int_{-\infty}^{\infty} dq_z \left[ \frac{1}{\varepsilon_q} \frac{\beta_{pq}^2}{|q_z \hat{\mathbf{z}} + \mathbf{k}_q|^2 - k_q^2} \left( \varepsilon_p^2 \{k_q^2 (\mathbf{I} - \hat{\mathbf{z}}\hat{\mathbf{z}}) - [\mathbf{k}_q]_{\perp} [\mathbf{k}_q]_{\perp}\} - \varepsilon_q \varepsilon_p (q_z + k_{qz}) (\hat{\mathbf{z}} [\mathbf{k}_q]_{\perp} + [\mathbf{k}_q]_{\perp} \hat{\mathbf{z}}) \right. \right. \\ &\quad \left. \left. + \varepsilon_q^2 |[\mathbf{k}_q]_{\perp}|^2 \hat{\mathbf{z}}\hat{\mathbf{z}} \right) \right] \tilde{\chi}_v(q_z) \\ &= \frac{\beta_{pq}^{(1D)2}}{2\pi \varepsilon_q} \int_{-\infty}^{\infty} dq_z \frac{\tilde{\chi}_v(q_z)}{|q_z \hat{\mathbf{z}} + \mathbf{k}_q|^2 - k_q^2} \left[ \varepsilon_p^2 (k_q \cos \theta)^2 \hat{\mathbf{x}}\hat{\mathbf{x}} + \varepsilon_q^2 (k_q \sin \theta)^2 \hat{\mathbf{z}}\hat{\mathbf{z}} - \varepsilon_q (k_q \sin \theta) \varepsilon_p (q_z + k_{qz}) (\hat{\mathbf{x}}\hat{\mathbf{z}} + \hat{\mathbf{z}}\hat{\mathbf{x}}) \right] \\ &\quad + \left( \frac{\beta_{pq}^{(1D)2}}{2\pi \varepsilon_q} \int_{-\infty}^{\infty} dq_z \frac{\tilde{\chi}_v(q_z)}{|q_z \hat{\mathbf{z}} + \mathbf{k}_q|^2 - k^2} \right) k^2 \varepsilon_p^2 \hat{\mathbf{y}}\hat{\mathbf{y}}. \end{aligned} \quad (\text{S34})$$

We obtain an explicit expression for the third-order term  $\mathcal{A}_3^{(p)}(\mathbf{k}_q)$  for stratified media. We simplify the integrand given in Eq. (S20) by substituting Eq. (S30), Eq. (S32), and Eq. (S33) into it and taking  $\mathbf{x} = \mathbf{k}_q + \mathbf{q}_1$  and  $\mathbf{y} = \mathbf{k}_q + \mathbf{q}_2$ :

$$\begin{aligned} &\left[ L_p^{(q)} \cdot \tilde{\mathbf{H}}^{(q)}(\mathbf{x}) \cdot L_p^{(q)} \cdot \tilde{\mathbf{H}}^{(q)}(\mathbf{y}) \right] \cdot L_p^{(q)} \\ &= \left( \frac{1}{\varepsilon_q} \frac{\beta_{pq}^2}{x^2 - k_q^2} \left[ \varepsilon_p^2 \{k_q^2 (\mathbf{I} - \hat{\mathbf{z}}\hat{\mathbf{z}}) - [\mathbf{x}]_{\perp} [\mathbf{x}]_{\perp}\} - \varepsilon_q \varepsilon_p x_z (\hat{\mathbf{z}} [\mathbf{x}]_{\perp} + [\mathbf{x}]_{\perp} \hat{\mathbf{z}}) + \varepsilon_q^2 (x^2 - x_z^2) \hat{\mathbf{z}}\hat{\mathbf{z}} \right] \right) \\ &\quad \cdot \frac{1}{\varepsilon_q} \left( \frac{k_q^2 \mathbf{I} - \mathbf{y}\mathbf{y}}{y^2 - k_q^2} + \hat{\mathbf{z}}\hat{\mathbf{z}} \right) \cdot \beta_{pq} [\varepsilon_p (\mathbf{I} - \hat{\mathbf{z}}\hat{\mathbf{z}}) + \varepsilon_q \hat{\mathbf{z}}\hat{\mathbf{z}}] \\ &= \frac{\beta_{pq}^{(1D)3}}{\varepsilon_q^2} \frac{1}{x^2 - k_q^2} \frac{1}{y^2 - k_q^2} \left[ \varepsilon_p^2 \{k_q^2 (\mathbf{I} - \hat{\mathbf{z}}\hat{\mathbf{z}}) - [\mathbf{x}]_{\perp} [\mathbf{x}]_{\perp}\} - \varepsilon_q \varepsilon_p x_z (\hat{\mathbf{z}} [\mathbf{x}]_{\perp} + [\mathbf{x}]_{\perp} \hat{\mathbf{z}}) + \varepsilon_q^2 (x^2 - x_z^2) \hat{\mathbf{z}}\hat{\mathbf{z}} \right] \\ &\quad \cdot \left\{ \varepsilon_p [k_q^2 (\mathbf{I} - \hat{\mathbf{z}}\hat{\mathbf{z}}) - \mathbf{y}[\mathbf{y}]_{\perp}] + \varepsilon_q [y^2 \hat{\mathbf{z}}\hat{\mathbf{z}} - \mathbf{y}y_z \hat{\mathbf{z}}] \right\} \\ &\quad + \varepsilon_p \varepsilon_q^2 [x_z y_z [\mathbf{x}]_{\perp} \cdot [\mathbf{y}]_{\perp} \hat{\mathbf{z}}\hat{\mathbf{z}} - x_z (y^2 - y_z^2) [\mathbf{x}]_{\perp} \hat{\mathbf{z}} - y_z (x^2 - x_z^2) \hat{\mathbf{z}} [\mathbf{y}]_{\perp}] + \varepsilon_q^3 (x^2 - x_z^2) (y^2 - y_z^2) \hat{\mathbf{z}}\hat{\mathbf{z}} \} \end{aligned} \quad (\text{S35})$$

Substituting Eq. (S29) and Eq. (S35) into Eq. (S20) yields

$$\begin{aligned}
\mathcal{A}_3^{(p)}(\mathbf{k}_q) &= \frac{-1}{\phi_p} \frac{\beta_{pq}^{(1D)^3}}{\varepsilon_q^2} \frac{(2\pi)^4}{(2\pi)^6} \int_{-\infty}^{\infty} dq_{1z} \int_{-\infty}^{\infty} dq_{2z} \frac{1}{|\mathbf{k}_q + q_{1z}\hat{\mathbf{z}}|^2 - k_q^2} \frac{1}{|\mathbf{k}_q + q_{2z}\hat{\mathbf{z}}|^2 - k_q^2} \\
&\quad \left( \varepsilon_p^3 \{k_q^4 (\mathbf{I} - \hat{\mathbf{z}}\hat{\mathbf{z}}) + (|\mathbf{k}_q|_{\perp}^2 - 2k_q^2) [\mathbf{k}_q]_{\perp} [\mathbf{k}_q]_{\perp} \} \right. \\
&\quad + \varepsilon_p^2 \varepsilon_q [ (|\mathbf{k}_q|_{\perp}^2 - k_q^2) (x_z \hat{\mathbf{z}} [\mathbf{k}_q]_{\perp} + y_z [\mathbf{k}_q]_{\perp} \hat{\mathbf{z}}) + x_z y_z [\mathbf{k}_q]_{\perp} [\mathbf{k}_q]_{\perp} ] \\
&\quad + \varepsilon_p \varepsilon_q^2 |\mathbf{k}|_{\perp}^2 [x_z y_z \hat{\mathbf{z}}\hat{\mathbf{z}} - x_z [\mathbf{k}_q]_{\perp} \hat{\mathbf{z}} - y_z \hat{\mathbf{z}} [\mathbf{k}_q]_{\perp}] + \varepsilon_q^3 |\mathbf{k}|_{\perp}^4 \hat{\mathbf{z}}\hat{\mathbf{z}} \Big) \tilde{\Delta}_3^{(p)}(q_{1z}, q_{2z}) \\
&= \frac{-1}{\phi_p} \frac{\beta_{pq}^{(1D)^3}}{(2\pi\varepsilon_q)^2} \int_{-\infty}^{\infty} dq_{1z} \int_{-\infty}^{\infty} dq_{2z} \frac{1}{|\mathbf{k}_q + q_{1z}\hat{\mathbf{z}}|^2 - k_q^2} \frac{1}{|\mathbf{k}_q + q_{2z}\hat{\mathbf{z}}|^2 - k_q^2} \\
&\quad \left( \varepsilon_p^3 \{k_q^4 (\mathbf{I} - \hat{\mathbf{z}}\hat{\mathbf{z}}) + (k_{qz}^2 - 2k_q^2) [\mathbf{k}_q]_{\perp} [\mathbf{k}_q]_{\perp} \} + \varepsilon_q^3 (k_q^2 - k_{qz}^2)^2 \hat{\mathbf{z}}\hat{\mathbf{z}} \right. \\
&\quad + \varepsilon_p^2 \varepsilon_q \{k_{qz}^2 [(q_{1z} + k_{qz}) \hat{\mathbf{z}} [\mathbf{k}_q]_{\perp} + (q_{2z} + k_{qz}) [\mathbf{k}_q]_{\perp} \hat{\mathbf{z}}] + (q_{1z} + k_{qz})(q_{2z} + k_{qz}) [\mathbf{k}_q]_{\perp} [\mathbf{k}_q]_{\perp} \} \\
&\quad + \varepsilon_p \varepsilon_q^2 (k_q^2 - k_{qz}^2) [(q_{1z} + k_{qz})(q_{2z} + k_{qz}) \hat{\mathbf{z}}\hat{\mathbf{z}} - (q_{1z} + k_{qz}) [\mathbf{k}_q]_{\perp} \hat{\mathbf{z}} - (q_{2z} + k_{qz}) \hat{\mathbf{z}} [\mathbf{k}_q]_{\perp}] \Big) \tilde{\Delta}_3^{(p)}(q_{1z}, q_{2z}).
\end{aligned} \tag{S36}$$

As shown in Eq. (S34) and Eq. (S36), the tensors  $\mathcal{A}_n^{(p)}(\mathbf{k}_q)$  can be decomposed into four independent components:  $\hat{\mathbf{y}}\hat{\mathbf{y}}$ ,  $\hat{\mathbf{x}}\hat{\mathbf{x}}$ ,  $(\hat{\mathbf{x}}\hat{\mathbf{z}} + \hat{\mathbf{z}}\hat{\mathbf{x}})$ , and  $\hat{\mathbf{z}}\hat{\mathbf{z}}$ . Similarly, the effective dynamic dielectric constant tensor  $\varepsilon_e(\mathbf{k}_q)$  [or  $L_e(\mathbf{k}_q)$ ] in Eq. (S16).

### C. Multiple-Scattering Approximations: Normal Incidence

In this subsection, we restrict ourselves to the case where the wave is incident normally into the media ( $\mathbf{k}_q = k_q \hat{\mathbf{z}}$  and  $[\mathbf{k}_q]_{\perp} = \mathbf{0}$ ), and thus the wave number  $k_q$  henceforth is an independent variable instead of  $\mathbf{k}_q$ , as we did in Ref. [15]. In this case, waves propagating in such anisotropic 3D media can be rigorously considered to be waves propagating in one-dimensional ( $d = 1$ ) systems and so we sometimes refer to them as 1D media. Then, the  $n$ th order coefficients given in Eq. (S34) and Eq. (S36) solely have the component of  $\mathbf{I} - \hat{\mathbf{z}}\hat{\mathbf{z}}$  ( $= \hat{\mathbf{x}}\hat{\mathbf{x}} + \hat{\mathbf{y}}\hat{\mathbf{y}}$ ), i.e.,  $\mathcal{A}_n^{(p)}(k_q) = (\varepsilon_p \beta_{pq}^{(1D)})^n A_n^{\perp}(k_q; \varepsilon_q) (\mathbf{I} - \hat{\mathbf{z}}\hat{\mathbf{z}})$ . For the first two coefficients  $A_2^{\perp}(k_q; \varepsilon_q)$  and  $A_3^{\perp}(k_q; \varepsilon_q)$ , their explicit expressions in Fourier space can be easily obtained by substituting the normal incidence condition (i.e.,  $[\mathbf{k}_q]_{\perp} = \mathbf{0}$  and  $|k_{qz}| = k_q$ ) into Eq. (S34) and Eq. (S36):

$$A_2^{\perp}(k_q; \varepsilon_q) \equiv \frac{F^{(1D)}(k_q)}{\varepsilon_q} = \frac{k_q^2}{2\pi\varepsilon_q} \int_{-\infty}^{\infty} dq \frac{\tilde{\chi}_V(q)}{(q + k_q)^2 - k_q^2} \tag{S37}$$

$$= \frac{k_q^2}{\pi\varepsilon_q} \text{p.v.} \int_0^{\infty} dq_z \frac{\tilde{\chi}_V(q_z)}{q_z^2 - (2k_q)^2} + \frac{ik_q}{4\varepsilon_q} [\tilde{\chi}_V(0) + \tilde{\chi}_V(2k_q)], \tag{S38}$$

$$A_3^{\perp}(k_q; \varepsilon_q) = \frac{-1}{\phi_p} \left( \frac{k_q^2}{2\pi\varepsilon_q} \right)^2 \int_{-\infty}^{\infty} dq_1 \frac{1}{(k_q + q_1)^2 - k_q^2} \int_{-\infty}^{\infty} dq_2 \frac{1}{(k_q + q_2)^2 - k_q^2} \tilde{\Delta}_3^{(p)}(q_1, q_2), \tag{S39}$$

where  $F^{(1D)}(k)$  is the nonlocal attenuation function for layered media. Since the inverse Fourier transform of  $[(k_q + q) - k_q^2]^{-1}$  is  $i \exp(ik_q(|z| - z))/ (2k_q)$ , we can rewrite the direct-space representations of Eq. (S38) and Eq. (S39) as follows, respectively:

$$A_2^{\perp}(k_q; \varepsilon_q) = \frac{1}{\varepsilon_q} F^{(1D)}(k_q) = \frac{ik_q}{2} \int_0^{\infty} dz \chi_V(z) (e^{2ik_q z} + 1), \tag{S40}$$

$$\begin{aligned}
A_3^{\perp}(k_q; \varepsilon_q) &= \frac{-1}{\phi_p} \left( \frac{k_q^2}{\varepsilon_q} \right)^2 \int_{-\infty}^{\infty} dz_{21} \frac{ie^{ik_q(|z_{21}| - z_{21})}}{2k_q} \int_{-\infty}^{\infty} dz_{32} \frac{ie^{ik_q(|z_{32}| - z_{32})}}{2k_q} \Delta_3^{(p)}(z_1, z_2, z_3) \\
&= \frac{-1}{\phi_p} \left( \frac{k_q^2}{\varepsilon_q} \right)^2 \int_{-\infty}^{\infty} dz_{21} \frac{ie^{ik_q(|z_{21}| - z_{21})}}{2k_q} \int_{-\infty}^{\infty} dz_{32} \frac{ie^{ik_q(|z_{32}| - z_{32})}}{2k_q} [S_2^{(p)}(z_{21}) S_2^{(p)}(z_{32}) - \phi_p S_3^{(p)}(z_{21}, z_{32} + z_{21})].
\end{aligned} \tag{S41}$$

Due to the symmetry of  $\mathcal{A}_n^{(p)}(k_q)$ , one can decompose the effective tensor  $\epsilon_e(k_q)$  into two orthogonal components  $\epsilon_e^\perp(k_q)$  and  $\epsilon_e^z(k_q)$  for the transverse and longitudinal polarizations, respectively, as follows:

$$\epsilon_e(k_q) = \epsilon_e^\perp(k_q) (\mathbf{I} - \hat{\mathbf{z}}\hat{\mathbf{z}}) + \epsilon_e^z(k_q) \hat{\mathbf{z}}\hat{\mathbf{z}}. \quad (\text{S42})$$

Substituting Eq. (S42) and Eq. (S31) into Eq. (S8) yields the left-handed side of Eq. (S16) for layered media

$$\phi_p \mathbf{L}_p^{(q)} \cdot \mathbf{L}_e(k_q)^{-1} \cdot \phi_p \mathbf{L}_p^{(q)} = \frac{(\phi_p \epsilon_p \beta_{pq}^{(1D)})^2}{\epsilon_q (\epsilon_e^\perp(k_q) / \epsilon_q - 1)} (\mathbf{I} - \hat{\mathbf{z}}\hat{\mathbf{z}}) + \frac{(\phi_p \epsilon_q \beta_{pq}^{(1D)})^2}{\epsilon_q (1 - \epsilon_q / \epsilon_e^z(k_q))} \hat{\mathbf{z}}\hat{\mathbf{z}} \quad (\text{S43})$$

$$= \phi_p \mathbf{L}_p^{(q)} - \left\{ [\epsilon_q \beta_{pq}^{(1D)}]^2 A_2^\perp(k_q; \epsilon_q) + [\epsilon_q \beta_{pq}^{(1D)}]^3 A_3^\perp(k_q; \epsilon_q) + \dots + [\epsilon_q \beta_{pq}^{(1D)}]^n A_n^\perp(k_q; \epsilon_q) \right\} (\mathbf{I} - \hat{\mathbf{z}}\hat{\mathbf{z}}). \quad (\text{S44})$$

Since the transverse component  $\mathbf{I} - \hat{\mathbf{z}}\hat{\mathbf{z}}$  and the longitudinal component  $\hat{\mathbf{z}}\hat{\mathbf{z}}$  are orthogonal, we decompose Eq. (S43) into two multiple-scattering approximations for 3D layered media:

$$\frac{(\phi_p \epsilon_p \beta_{pq}^{(1D)})^2}{\epsilon_e^\perp(k_q) - \epsilon_q} = \phi_p \epsilon_p \beta_{pq}^{(1D)} - A_2^\perp(k_q; \epsilon_q) (\epsilon_p \beta_{pq}^{(1D)})^2 - A_3^\perp(k_q; \epsilon_q) (\epsilon_p \beta_{pq}^{(1D)})^3 - \dots - A_n^\perp(k_q; \epsilon_q) (\epsilon_p \beta_{pq}^{(1D)})^n, \quad (\text{S45})$$

$$\frac{(\phi_p \epsilon_q \beta_{pq}^{(1D)})^2}{\epsilon_q [1 - \epsilon_q / \epsilon_e^z(k_q)]} = \phi_p \epsilon_q \beta_{pq}^{(1D)}. \quad (\text{S46})$$

Note that because  $A_n^\perp(k_q; \epsilon_q)$  are complex-valued functions of wave number  $k_q, \epsilon_e^\perp(k_q)$  in Eq. (S45) are also complex-valued, implying that the media are effectively lossy due to scatterings from inhomogeneities. By contrast,  $\epsilon_e^z(k_q)$  is independent of  $k_q$ , reflecting the fact that a traveling longitudinal wave cannot exist for normally incident waves. We call Eq. (S45) *non-scaled* strong-contrast approximation that takes either phase 1 or 2 as the reference phase, i.e.,  $q = 1, 2$ . In Sec. 4, we derive the scaled variant of Eq. (S45) by renormalizing it with the optimal reference phase.

#### D. Perfect Transparency at the Three-Point Level

In section 4 of the main text, we analytically show that the finite perfect transparency interval [Eq. (32)] for stealthy hyperuniform layered systems (or, equivalently, 1D stealthy hyperuniform systems) with  $\tilde{\chi}_v(k) = 0$  for  $k < K$  is exact through the third-order terms. There, we outline the proof of a perfect transparency condition related to the third-order term  $A_3^\perp$ ; see Eq. (32) of the main text. Here, we provide a detailed proof of Eq. (32) of the main text.

Without losing generality, we can rewrite the third-order condition [Eq. (32)] as follows:

$$\text{Im}[A_3^\perp(k; 1)] = 0, \quad (k < K/2). \quad (\text{S47})$$

Substituting Eq. (S25) into the Fourier representation of  $A_3^\perp$  [Eq. (S39)] allows us to separate the third-order coefficient into three terms:

$$\begin{aligned} A_3^\perp(k; 1) &= \frac{-1}{\phi_p} \left( \frac{k^2}{2\pi} \right)^2 \int_{-\infty}^{\infty} dq_1 \int_{-\infty}^{\infty} dq_2 \frac{1}{(k+q_1)^2 - k^2} \frac{1}{(k+q_2)^2 - k^2} \left[ \tilde{\chi}_v(q_1) \tilde{\chi}_v(q_2) - \phi_p^2 (2\pi) \delta(q_1 - q_2) \tilde{\chi}_v(q_2) \right. \\ &\quad \left. - \phi_p \langle \tilde{\mathcal{J}}^{(p)}(-q_1) \tilde{\mathcal{J}}^{(p)}(q_1 - q_2) \tilde{\mathcal{J}}^{(p)}(q_2) \rangle \right] \\ &= \frac{-1}{\phi_p} \frac{k^4}{(2\pi)^2} \left\{ C_1^\perp(k) - \phi_p^2 (2\pi) C_2^\perp(k) - \phi_p C_3^\perp(k) \right\}, \end{aligned} \quad (\text{S48})$$

where  $C_1^\perp(k)$  and  $C_2^\perp(k)$  depend on the two-point statistics, whereas  $C_3^\perp(k)$  depends on the three-point statistics:

$$C_1^\perp(k) \equiv \left[ \frac{2\pi}{k^2} F^{(1D)}(k) \right]^2, \quad (\text{S49})$$

$$C_2^\perp(k) \equiv \int_{-\infty}^{\infty} dq_1 \left[ \frac{1}{(k+q_1)^2 - k^2} \right]^2 \tilde{\chi}_v(q_1), \quad (\text{S50})$$

$$C_3^\perp(k) \equiv \int_{-\infty}^{\infty} dq_1 \int_{-\infty}^{\infty} dq_2 \frac{1}{(k+q_1)^2 - k^2} \frac{1}{(k+q_2)^2 - k^2} \langle \tilde{\mathcal{J}}^{(p)}(q_1) \tilde{\mathcal{J}}^{(p)}(-q_1 + q_2) \tilde{\mathcal{J}}^{(p)}(-q_2) \rangle. \quad (\text{S51})$$

Therefore, we can prove Eq. (S47) by showing that for  $n = 1, 2, 3$ ,

$$\text{Im}[C_n^\perp(k)] = 0 \quad (k < K/2), \quad (\text{S52})$$

where  $C_n^\perp(k)$  are defined in Eq. (S49)-Eq. (S51), respectively.

To prove Eq. (S52), we utilize the three general properties of  $\tilde{\mathcal{J}}^{(p)}(k)$  for 1D disordered stealthy hyperuniform two-phase media:

$$\text{Stealthy hyperuniform condition: } \left| \tilde{\mathcal{J}}^{(p)}(k) \right| = 0, \quad \text{for } 0 \leq |k| < K, \quad (\text{S53})$$

$$\text{No Bragg peaks: } \left| \tilde{\mathcal{J}}^{(p)}(k) \right| < C, \quad \text{for any } k, \quad (\text{S54})$$

$$\text{Large-}k \text{ scaling from Eq. (S3): } \left| \tilde{\mathcal{J}}^{(p)}(k) \right| \leq \frac{C'}{|k|}, \quad \text{for } Q \leq |k|, \quad (\text{S55})$$

where  $C'$  and  $C$  are some finite positive numbers, and  $Q$  is a large wave number much greater than  $K$ .

One can immediately see that Eq. (S52) is true for  $n = 1$ . For  $k < K/2$ , Eq. (S38) gives  $\text{Im}[F^{(1D)}(k)] = 0$ , and thus  $\text{Im}[C_1^\perp(k)] = 0$ . We then prove Eq. (S52) for  $n = 2$ . The integrand in Eq. (S50) is real-valued and nonnegative except at two singular points ( $q_1 = 0$  and  $-2k$ ) because it is the product of the spectral density  $\tilde{\chi}_v(q_1)$  and the square of the Green's function [i.e.,  $(|k + q_1|^2 - k^2)^{-2}$ ]. For  $k < K/2$ , however, this integrand has no singularity because the stealthy hyperuniform condition [Eq. (S53)] can completely remove these two singular points that the Green's function can arise. Furthermore, due to the properties of  $\tilde{\chi}_v(k)$  [Eq. (S54) and Eq. (S55)], this nonnegative integrand of Eq. (S50) is bounded from above and decays rapidly like  $|q_1|^{-6}$  for large  $|q_1|$ . Therefore, for  $k < K/2$ , the real-valued integrand of Eq. (S50) is absolutely integrable, leading to  $\text{Im}[C_2^\perp(k)] = 0$ .

We then prove Eq. (S52) for  $n = 3$ . The crucial part of the proof is to show that for  $k < K/2$ , the integrand in Eq. (S51) is absolutely integrable (i.e., the integral of its absolute value is well-defined and finite) such that the Fubini-Tonelli theorem [16] enables one to interchange the integration order in Eq. (S51). Once we show the integration order is interchangeable, using the general property of the Fourier transform [i.e.,  $\tilde{\mathcal{J}}^{(p)}(k')^* = \tilde{\mathcal{J}}^{(p)}(-k')$ ], we can immediately show that for  $k < K/2$ ,  $C_3^\perp(k)$  is real-valued because

$$\begin{aligned} [C_3^\perp(k)]^* &= \int_{-\infty}^{\infty} dq_1 \int_{-\infty}^{\infty} dq_2 \frac{1}{(k + q_1)^2 - k^2} \frac{1}{(k + q_2)^2 - k^2} \langle [\tilde{\mathcal{J}}^{(p)}(q_1) \tilde{\mathcal{J}}^{(p)}(-q_1 + q_2) \tilde{\mathcal{J}}^{(p)}(-q_2)]^* \rangle \\ &= \int_{-\infty}^{\infty} dq_1 \int_{-\infty}^{\infty} dq_2 \frac{1}{(k + q_1)^2 - k^2} \frac{1}{(k + q_2)^2 - k^2} \langle \tilde{\mathcal{J}}^{(p)}(-q_1) \tilde{\mathcal{J}}^{(p)}(q_1 - q_2) \tilde{\mathcal{J}}^{(p)}(q_2) \rangle \end{aligned} \quad (\text{S56})$$

$$= \int_{-\infty}^{\infty} dq_2 \int_{-\infty}^{\infty} dq_1 \frac{1}{(k + q_2)^2 - k^2} \frac{1}{(k + q_1)^2 - k^2} \langle \tilde{\mathcal{J}}^{(p)}(q_2) \tilde{\mathcal{J}}^{(p)}(-q_2 + q_1) \tilde{\mathcal{J}}^{(p)}(-q_1) \rangle \quad (\text{S57})$$

$$= C_3^\perp(k), \quad (\text{S58})$$

where we have changed the integration order from Eq. (S56) to Eq. (S57).

Now let us show that the integrand in Eq. (S51) is absolutely integrable if  $k < K/2$ . We first reduce the absolute value of this integrand in a simpler form:

$$\begin{aligned} & \left| \frac{1}{(k + q_1)^2 - k^2} \frac{1}{(k + q_2)^2 - k^2} \langle \tilde{\mathcal{J}}^{(p)}(q_1) \tilde{\mathcal{J}}^{(p)}(-q_1 + q_2) \tilde{\mathcal{J}}^{(p)}(-q_2) \rangle \right| \\ & \leq \left| \frac{1}{(k + q_1)^2 - k^2} \frac{1}{(k + q_2)^2 - k^2} \right| \left| \langle \tilde{\mathcal{J}}^{(p)}(q_1) \tilde{\mathcal{J}}^{(p)}(-q_1 + q_2) \tilde{\mathcal{J}}^{(p)}(-q_2) \rangle \right| \\ & = \left| \frac{1}{(k + q_1)^2 - k^2} \right| \left| \frac{1}{(k + q_2)^2 - k^2} \right| \left| \langle \tilde{\mathcal{J}}^{(p)}(q_1) \tilde{\mathcal{J}}^{(p)}(-q_1 + q_2) \tilde{\mathcal{J}}^{(p)}(-q_2) \rangle \right| \\ & \leq \left| \frac{1}{(k + q_1)^2 - k^2} \right| \left| \frac{1}{(k + q_2)^2 - k^2} \right| C \left| \langle \tilde{\mathcal{J}}^{(p)}(q_1) \tilde{\mathcal{J}}^{(p)}(-q_2) \rangle \right|, \end{aligned} \quad (\text{S59})$$

where we have used Eq. (S54). If the integral of Eq. (S59) is bounded from above by a finite constant, then we prove that the integrand in Eq. (S51) is absolutely integrable.

$$\begin{aligned} & \int_{-\infty}^{\infty} dq_1 \int_{-\infty}^{\infty} dq_2 \left| \frac{1}{(k+q_1)^2 - k^2} \right| \left| \frac{1}{(k+q_2)^2 - k^2} \right| C \left\langle \left| \tilde{\mathcal{J}}^{(p)}(q_1) \right| \left| \tilde{\mathcal{J}}^{(p)}(-q_2) \right| \right\rangle \\ &= C \left\langle \int_{-\infty}^{\infty} dq_1 \int_{-\infty}^{\infty} dq_2 \frac{\left| \tilde{\mathcal{J}}^{(p)}(q_1) \right| \left| \tilde{\mathcal{J}}^{(p)}(-q_2) \right|}{|(k+q_1)^2 - k^2| |(k+q_2)^2 - k^2|} \right\rangle = C \left\langle \left[ \int_{-\infty}^{\infty} dq_1 \frac{\left| \tilde{\mathcal{J}}^{(p)}(q_1) \right|}{|(k+q_1)^2 - k^2|} \right]^2 \right\rangle. \end{aligned} \quad (\text{S60})$$

We then compute the integral that appears in the upper bound, Eq. (S60):

$$\begin{aligned} & \int_{-\infty}^{\infty} dq_1 \frac{\left| \tilde{\mathcal{J}}^{(p)}(q_1) \right|}{|(k+q_1)^2 - k^2|} \\ &= \int_{|q_1| < K} dq_1 \frac{\left| \tilde{\mathcal{J}}^{(p)}(q_1) \right|}{|(k+q_1)^2 - k^2|} + \int_{K \leq |q_1| < Q} dq_1 \frac{\left| \tilde{\mathcal{J}}^{(p)}(q_1) \right|}{|(k+q_1)^2 - k^2|} + \int_{Q \leq |q_1|} dq_1 \frac{\left| \tilde{\mathcal{J}}^{(p)}(q_1) \right|}{|(k+q_1)^2 - k^2|} \\ &\leq 0 + \int_{K \leq |q_1| < Q} dq_1 \frac{C}{|(k+q_1)^2 - k^2|} + \int_{Q \leq |q_1|} dq_1 \frac{C'/|q_1|}{|(k+q_1)^2 - k^2|}, \end{aligned} \quad (\text{S61})$$

where we have applied Eq. (S53)-Eq. (S55) sequentially in the three integrals. It is important to note that the first integral over  $-K < q_1 < K$  is divergent if the system is not stealthy hyperuniform. The second integral in Eq. (S61) is positive and bounded from above, as shown below:

$$\int_{K \leq |q_1| < Q} dq_1 \frac{C}{|(k+q_1)^2 - k^2|} \leq 2C \int_{-Q}^{-K} dq_1 \frac{1}{q_1(q_1 + 2k)} = \frac{C}{k} \ln \left( \frac{K}{K - 2k} \frac{Q - 2k}{Q} \right). \quad (\text{S62})$$

The third integral in Eq. (S61) is also positive and bounded from above, as shown below:

$$\int_{Q \leq |q_1|} dq_1 \frac{C'/|q_1|}{|(k+q_1)^2 - k^2|} \leq 2C' \int_{-\infty}^{-Q} dq_1 \frac{-1}{q_1^2(q_1 + 2k)} = \frac{-C'}{k} \left[ \frac{1}{Q} + \frac{1}{2k} \ln \left( 1 - \frac{2k}{Q} \right) \right]. \quad (\text{S63})$$

Combining Eq. (S58)-Eq. (S63) shows that the integrand in Eq. (S51) is absolutely integrable, i.e.,

$$\begin{aligned} & \int_{-\infty}^{\infty} dq_1 \int_{-\infty}^{\infty} dq_2 \left| \frac{1}{(k+q_1)^2 - k^2} \frac{1}{(k+q_2)^2 - k^2} \right| \left\langle \tilde{\mathcal{J}}^{(p)}(q_1) \tilde{\mathcal{J}}^{(p)}(-q_1 + q_2) \tilde{\mathcal{J}}^{(p)}(-q_2) \right\rangle \\ &\leq C \left\{ \frac{C}{k} \ln \left( \frac{K}{K - 2k} \frac{Q - 2k}{Q} \right) + \frac{-C'}{k} \left[ \frac{1}{Q} + \frac{1}{2k} \ln \left( 1 - \frac{2k}{Q} \right) \right] \right\}^2. \end{aligned} \quad (\text{S64})$$

Therefore, as noted in Eq. (S58), Eq. (S52) for  $n = 3$  is true.

**Remarks:**

1. The condition, Eq. (S52), for  $n = 2$  can be shown alternatively from the following relation:

$$\begin{aligned} C_2^\perp(k_q) &= \int_{-\infty}^{\infty} dq \left[ \frac{1}{(k+q)^2 - k^2} \right]^2 \tilde{\chi}_v(q) = \frac{1}{(2k)^2} \int_{-\infty}^{\infty} dq \left[ \frac{1}{q^2} + \frac{1}{(q+2k)^2} - \frac{2}{(k+q)^2 - k^2} \right] \tilde{\chi}_v(q) \\ &= \frac{1}{(2k)^2} \int_{-\infty}^{\infty} dq \left[ \frac{1}{q^2} + \frac{1}{(q+2k)^2} \right] \tilde{\chi}_v(q) - \frac{\pi}{k^4} F^{(1D)}(k) \\ &= \frac{1}{(2k)^2} \left\{ \text{p.v.} \int_{-\infty}^{\infty} dq \frac{\tilde{\chi}_v(q)}{q^2} + \text{p.v.} \int_{-\infty}^{\infty} dq \frac{\tilde{\chi}_v(q)}{(q+2k)^2} + i\pi \left[ \frac{d\tilde{\chi}_v(0)}{dq} + \frac{d\tilde{\chi}_v(2k)}{dq} \right] \right\} - \frac{\pi}{k^4} F^{(1D)}(k), \end{aligned} \quad (\text{S65})$$

where we have used the Cauchy differential formula [17]:

$$\int_{-\infty}^{\infty} dz \frac{f(z)}{(z-a)^{n+1}} = \text{p.v.} \int_{-\infty}^{\infty} dz \frac{f(z)}{(z-a)^{n+1}} + \frac{i\pi}{n!} f^{(n)}(a), \quad n = 0, 1, 2, \dots,$$

and  $f(z)$  is an analytic function, and  $f^{(n)}(a)$  is its  $n$ th-order derivative at  $z = a$ . For stealthy hyperuniform media,  $\tilde{\chi}_v(k) = 0$  for  $k < K$ , and thus its derivative is also zero. Thus, Eq. (S50) yields that  $\text{Im}[C_2^\perp(k)] = 0$  for  $k < K/2$ .

### 3. NONLOCAL STRONG-CONTRAST EXPANSIONS FOR TRANSVERSELY ISOTROPIC MEDIA

Here, we derive the multiple scattering approximations of  $\epsilon_e(\mathbf{k}_q)$  suited for 3D transversely isotropic two-phase media from the general strong-contrast expansion given in Eq. (S6). We begin by describing how to utilize the symmetries of transversely isotropic media in the series. We then truncate the resulting series at the  $n$ -point level for extracting multiple-scattering approximations.

#### A. Symmetries of Transversely Isotropic Media

A transversely isotropic medium is translationally invariant along one axis and statistically isotropic around this axis. In the present work, we take the  $z$  axis as the symmetry axis of the transversely isotropic media, as shown in Fig. 1(b) of the main text. Due to the symmetries, the  $n$ -point correlation functions are independent of  $z$  coordinates of relative positions and dependent on horizontal distances of relative positions:  $S_n^{(p)}(\mathbf{x}_1, \dots, \mathbf{x}_n) = S_n^{(p)}([\mathbf{x}_2 - \mathbf{x}_1]_\perp, [\mathbf{x}_3 - \mathbf{x}_1]_\perp, \dots, [\mathbf{x}_n - \mathbf{x}_1]_\perp)$ , where  $[\mathbf{x}]_\perp \equiv \mathbf{x} \cdot (\mathbf{I} - \hat{\mathbf{z}}\hat{\mathbf{z}})$ . Consequently, the corresponding spectral density or the Fourier transform of  $\Delta_n^{(p)}(\mathbf{x}_1, \dots, \mathbf{x}_n)$  given in Eq. (S11) can be simplified as follows:

$$\tilde{\chi}_V(\mathbf{q}) = \tilde{\chi}_V(q_\perp) (2\pi) \delta(q_z), \quad (\text{S66})$$

$$\tilde{\Delta}_n^{(p)}(\mathbf{q}_1, \dots, \mathbf{q}_{n-1}) = (2\pi)^{n-1} \delta(q_{1z}) \dots \delta(q_{n-1z}) \tilde{\Delta}_n^{(p)}([\mathbf{q}_1]_\perp, \dots, [\mathbf{q}_{n-1}]_\perp), \quad n = 3, \dots, \quad (\text{S67})$$

where  $q_\perp \equiv \sqrt{q_x^2 + q_y^2}$ , and  $\tilde{\chi}_V(q_\perp)$  is the radial spectral density of the 2D statistically isotropic media, from which the transversely isotropic media are derived.

Because of the invariance along the  $z$ -axis, it is appropriate to choose a needle-like exclusion volume aligned along the  $z$  axis, which gives

$$\mathbf{D}^{(q)} = \frac{1}{2\epsilon_q} (\mathbf{I} - \hat{\mathbf{z}}\hat{\mathbf{z}}), \quad (\text{S68})$$

$$\mathbf{L}^{(q)} = (\epsilon_p - \epsilon_q) \hat{\mathbf{z}}\hat{\mathbf{z}} + 2\epsilon_q \frac{\epsilon_p - \epsilon_q}{\epsilon_p + \epsilon_q} (\mathbf{I} - \hat{\mathbf{z}}\hat{\mathbf{z}}) = \beta_{pq}^{(2D)} [(\epsilon_p + \epsilon_q) \hat{\mathbf{z}}\hat{\mathbf{z}} + 2\epsilon_q (\mathbf{I} - \hat{\mathbf{z}}\hat{\mathbf{z}})], \quad (\text{S69})$$

where we have obtained the expansion parameter [Eq. (S69)] by substituting Eq. (S68) into Eq. (S7), and  $\beta_{pq}^{(2D)} \equiv (\epsilon_p - \epsilon_q)/(\epsilon_q + \epsilon_p)$  is the 2D *dielectric polarizability*. Then, using Eq. (S68) and Eq. (S69), we rewrite Eq. (S18) as

$$\tilde{\mathbf{H}}^{(q)}(\mathbf{k}) = \frac{1}{\epsilon_q} \left[ \frac{k^2 \mathbf{I} - \mathbf{k}\mathbf{k}}{k^2 - k_q^2} + \frac{1}{2} (\mathbf{I} - \hat{\mathbf{z}}\hat{\mathbf{z}}) \right] = \frac{1}{2\epsilon_q} \frac{(k^2 + k_q^2)(\mathbf{I} - \hat{\mathbf{z}}\hat{\mathbf{z}}) + 2k^2 \hat{\mathbf{z}}\hat{\mathbf{z}} - 2\mathbf{k}\mathbf{k}}{k^2 - k_q^2}. \quad (\text{S70})$$

#### B. Multiple-Scattering Approximations: General Cases

Using Eq. (S68), Eq. (S69), and Eq. (S70), we derive explicit expressions for the first two coefficients  $\mathcal{A}_n^{(p)}(\mathbf{k}_q)$  for  $n = 2, 3$  in transversely isotropic media. Without losing generality, we assume an obliquely incident wavevector  $\mathbf{k}_q = k_q(\hat{\mathbf{z}} \sin \theta + \hat{\mathbf{y}} \cos \theta)$ , where  $\theta$  is the incidence angle.

As we did in Sec. S2B, we derive the following expressions from Eq. (S70) and Eq. (S69):

$$\begin{aligned} \tilde{\mathbf{H}}^{(q)}(\mathbf{Y}) \cdot \mathbf{L}_p^{(q)} &= \frac{\beta_{pq}^{(2D)}}{2\epsilon_q} \frac{1}{Y^2 - k_q^2} \left( (2\epsilon_q)(Y^2 + k_q^2)(\mathbf{I} - \hat{\mathbf{z}}\hat{\mathbf{z}}) + (\epsilon_q + \epsilon_p)2k_q^2 \hat{\mathbf{z}}\hat{\mathbf{z}} - 2\mathbf{Y}\{2\epsilon_q[\mathbf{Y}]_\perp + (\epsilon_p + \epsilon_q)Y_z \hat{\mathbf{z}}\} \right) \\ &= \frac{\beta_{pq}^{(2D)}}{2\epsilon_q} \frac{1}{Y^2 - k_q^2} \left( (2\epsilon_q)[(Y^2 + k_q^2)(\mathbf{I} - \hat{\mathbf{z}}\hat{\mathbf{z}}) - 2\mathbf{Y}[\mathbf{Y}]_\perp] + (\epsilon_q + \epsilon_p)2[k_q^2 \hat{\mathbf{z}}\hat{\mathbf{z}} - \mathbf{Y}Y_z \hat{\mathbf{z}}] \right), \end{aligned} \quad (\text{S71})$$

$$\begin{aligned} \mathbf{L}_p^{(q)} \cdot \tilde{\mathbf{H}}^{(q)}(\mathbf{X}) \cdot \mathbf{L}_p^{(q)} &= \frac{[\beta_{pq}^{(2D)}]^2}{2\epsilon_q} \frac{1}{X^2 - k_q^2} \left( (2\epsilon_q)^2(X^2 + k_q^2)(\mathbf{I} - \hat{\mathbf{z}}\hat{\mathbf{z}}) + (\epsilon_q + \epsilon_p)^2 2k_q^2 \hat{\mathbf{z}}\hat{\mathbf{z}} \right. \\ &\quad \left. - 2\{2\epsilon_q[\mathbf{X}]_\perp + (\epsilon_p + \epsilon_q)X_z \hat{\mathbf{z}}\} \{2\epsilon_q[\mathbf{X}]_\perp + (\epsilon_p + \epsilon_q)X_z \hat{\mathbf{z}}\} \right) \\ &= \frac{[\beta_{pq}^{(2D)}]^2}{2\epsilon_q} \frac{1}{X^2 - k_q^2} \left( (2\epsilon_q)^2[(X^2 + k_q^2)(\mathbf{I} - \hat{\mathbf{z}}\hat{\mathbf{z}}) - 2[\mathbf{X}]_\perp[\mathbf{X}]_\perp] - 2(2\epsilon_q)(\epsilon_p + \epsilon_q)X_z([\mathbf{X}]_\perp \hat{\mathbf{z}} + \hat{\mathbf{z}}[\mathbf{X}]_\perp) \right. \\ &\quad \left. + (\epsilon_q + \epsilon_p)^2 2(k_q^2 - X_z^2) \hat{\mathbf{z}}\hat{\mathbf{z}} \right), \end{aligned} \quad (\text{S72})$$

$$\begin{aligned}
& \mathbf{L}_p^{(q)} \cdot \tilde{\mathbf{H}}^{(q)}(\mathbf{X}) \cdot \mathbf{L}_p^{(q)} \cdot \tilde{\mathbf{H}}^{(q)}(\mathbf{Y}) \cdot \mathbf{L}_p^{(q)} \\
&= \frac{[\beta_{pq}^{(2D)}]^3}{(2\varepsilon_q)^2} \frac{1}{X^2 - k_q^2} \frac{1}{Y^2 - k_q^2} \left( (2\varepsilon_q)^3 \{ (X^2 + k_q^2) [ (Y^2 + k_q^2)(\mathbf{I} - \hat{\mathbf{z}}\hat{\mathbf{z}}) - 2[\mathbf{Y}]_{\perp}[\mathbf{Y}]_{\perp} ] \right. \\
&\quad - 2(Y^2 + k_q^2)[\mathbf{X}]_{\perp}[\mathbf{X}]_{\perp} + 4([\mathbf{X}]_{\perp} \cdot [\mathbf{Y}]_{\perp})[\mathbf{X}]_{\perp}[\mathbf{Y}]_{\perp} \} \\
&\quad + (2\varepsilon_q)^2(\varepsilon_p + \varepsilon_q) \{ -2(X^2 + k_q^2)[\mathbf{Y}]_{\perp}Y_z\hat{\mathbf{z}} - 2(Y^2 + k_q^2)X_z\hat{\mathbf{z}}[\mathbf{X}]_{\perp} + 4X_zY_z[\mathbf{X}]_{\perp}[\mathbf{Y}]_{\perp} \\
&\quad + 4([\mathbf{X}]_{\perp} \cdot [\mathbf{Y}]_{\perp})(X_z\hat{\mathbf{z}}[\mathbf{Y}]_{\perp} + [\mathbf{X}]_{\perp}Y_z\hat{\mathbf{z}}) \} \\
&\quad + (2\varepsilon_q)(\varepsilon_p + \varepsilon_q)^2 \{ 4[-k_q^2X_z\hat{\mathbf{z}}[\mathbf{X}]_{\perp} + Y_z^2X_z[\mathbf{X}]_{\perp}\hat{\mathbf{z}} - (k^2 - X_z^2)Y_z\hat{\mathbf{z}}[\mathbf{Y}]_{\perp} + ([\mathbf{X}]_{\perp} \cdot [\mathbf{Y}]_{\perp})X_zY_z\hat{\mathbf{z}} \} \\
&\quad \left. + 4(\varepsilon_p + \varepsilon_q)^3(k_q^2 - X_z^2)(k_q^2 - Y_z^2)\hat{\mathbf{z}}\hat{\mathbf{z}} \right), \tag{S73}
\end{aligned}$$

147 where we have taken  $\mathbf{X} = \mathbf{k}_q + \mathbf{q}_1$  and  $\mathbf{Y} = \mathbf{k}_q + \mathbf{q}_2$ .

We obtain expression for  $\mathcal{A}_2^{(p)}(\mathbf{k}_q)$  by substituting Eq. (S66) and Eq. (S72) into Eq. (S19):

$$\begin{aligned}
\mathcal{A}_2^{(p)}(\mathbf{k}_q) &= \frac{[\beta_{pq}^{(2D)}]^2}{2\varepsilon_q} \frac{1}{(2\pi)^2} \int_{\mathbb{R}^2} \frac{d\mathbf{q}_{\perp}}{|\mathbf{k}_q + \mathbf{q}_{\perp}|^2 - k_q^2} \left[ (2\varepsilon_q)^2 [ (|\mathbf{k}_q + \mathbf{q}_{\perp}|^2 + k_q^2)(\mathbf{I} - \hat{\mathbf{z}}\hat{\mathbf{z}}) - 2([\mathbf{k}_q]_{\perp} + \mathbf{q}_{\perp})([\mathbf{k}_q]_{\perp} + \mathbf{q}_{\perp}) ] \right. \\
&\quad \left. - 2(2\varepsilon_q)(\varepsilon_p + \varepsilon_q)(k_{q_z})([\mathbf{k}_q]_{\perp} + \mathbf{q}_{\perp})\hat{\mathbf{z}} + \hat{\mathbf{z}}([\mathbf{k}_q]_{\perp} + \mathbf{q}_{\perp}) + (\varepsilon_q + \varepsilon_p)^2 2(k_q^2 - k_{q_z}^2)\hat{\mathbf{z}}\hat{\mathbf{z}} \right] \tilde{\chi}_V(q_{\perp}) \\
&= \frac{[\beta_{pq}^{(2D)}]^2}{2\varepsilon_q} \frac{1}{(2\pi)^2} \int_{\mathbb{R}^2} \frac{d\mathbf{q}_{\perp}}{|\mathbf{k}_q + \mathbf{q}_{\perp}|^2 - k_q^2} \left\{ (2\varepsilon_q)^2 [ (|\mathbf{k}_q + \mathbf{q}_{\perp}|^2 + k_q^2)(\mathbf{I} - \hat{\mathbf{z}}\hat{\mathbf{z}}) - 2([\mathbf{k}_q]_{\perp} + \mathbf{q}_{\perp})([\mathbf{k}_q]_{\perp} + \mathbf{q}_{\perp}) ] \right. \\
&\quad \left. - 2(2\varepsilon_q)(\varepsilon_p + \varepsilon_q)(k_{q_z})(k_q \cos \theta + q_{\perp} \cos \phi)(\hat{\mathbf{y}}\hat{\mathbf{z}} + \hat{\mathbf{z}}\hat{\mathbf{y}}) + (\varepsilon_q + \varepsilon_p)^2 2(k_q \cos \theta)^2 \hat{\mathbf{z}}\hat{\mathbf{z}} \right\} \tilde{\chi}_V(q_{\perp}). \tag{S74}
\end{aligned}$$

Similarly, we obtain expression for  $\mathcal{A}_3^{(p)}(\mathbf{k}_q)$  by substituting Eq. (S67) and Eq. (S73) into Eq. (S20):

$$\begin{aligned}
\mathcal{A}_3^{(p)}(\mathbf{k}_q) &= \left( \frac{-1}{\phi_p} \right) \frac{[\beta_{pq}^{(2D)}]^3}{(2\varepsilon_q)^2} \frac{1}{(2\pi)^4} \int_{\mathbb{R}^2} d\mathbf{q}_1 d\mathbf{q}_2 \frac{\tilde{\Delta}_3^{(p)}(-\mathbf{q}_1, -\mathbf{q}_2)}{|\mathbf{k}_q + \mathbf{q}_1|^2 - k_q^2} \frac{1}{|\mathbf{k}_q + \mathbf{q}_2|^2 - k_q^2} \times \\
&\quad \left( (2\varepsilon_q)^3 \{ (X^2 + k_q^2) [ (Y^2 + k_q^2)(\mathbf{I} - \hat{\mathbf{z}}\hat{\mathbf{z}}) - 2[\mathbf{Y}]_{\perp}[\mathbf{Y}]_{\perp} ] - 2(Y^2 + k_q^2)[\mathbf{X}]_{\perp}[\mathbf{X}]_{\perp} + 4([\mathbf{X}]_{\perp} \cdot [\mathbf{Y}]_{\perp})[\mathbf{X}]_{\perp}[\mathbf{Y}]_{\perp} \} \right. \\
&\quad + (2\varepsilon_q)^2(\varepsilon_p + \varepsilon_q) \{ -2(X^2 + k_q^2)[\mathbf{Y}]_{\perp}Y_z\hat{\mathbf{z}} - 2(Y^2 + k_q^2)X_z\hat{\mathbf{z}}[\mathbf{X}]_{\perp} \\
&\quad + (2\varepsilon_q)(\varepsilon_p + \varepsilon_q)^2 \{ 4[-k_q^2X_z\hat{\mathbf{z}}[\mathbf{X}]_{\perp} + Y_z^2X_z[\mathbf{X}]_{\perp}\hat{\mathbf{z}} - (k_q^2 - X_z^2)Y_z\hat{\mathbf{z}}[\mathbf{Y}]_{\perp} + ([\mathbf{X}]_{\perp} \cdot [\mathbf{Y}]_{\perp})X_zY_z\hat{\mathbf{z}} \} \\
&\quad \left. + 4(\varepsilon_p + \varepsilon_q)^3(k_q^2 - X_z^2)(k_q^2 - Y_z^2)\hat{\mathbf{z}}\hat{\mathbf{z}} \right), \tag{S75}
\end{aligned}$$

148 where  $\mathbf{X} \equiv \mathbf{k}_q + \mathbf{q}_1$  and  $\mathbf{Y} \equiv \mathbf{k}_q + \mathbf{q}_2$ .

### 149 C. Multiple-Scattering Approximations: Normal Incidence

In this subsection, we restrict ourselves to the case where the wave is incident normally into the media (i.e.,  $\mathbf{k}_q = k_q \hat{\mathbf{y}}$  and  $k_{q_z} \equiv \mathbf{k}_q \cdot \hat{\mathbf{z}} = 0$ ), and thus the wave number  $k_q$  henceforth is an independent variable instead of  $\mathbf{k}_q$ . In this case, such waves propagating in transversely isotropic 3D media can be rigorously considered to be waves propagating in two-dimensional (2D) ( $d = 2$ ) systems, and so we sometimes refer to them as 2D media. Due to the statistical isotropy around the  $z$ -axis, the effective dielectric constant can be decomposed for TE and TM polarizations:

$$\varepsilon_e(k_q) = \varepsilon_e^{TE}(k_q)(\mathbf{I} - \hat{\mathbf{z}}\hat{\mathbf{z}}) + \varepsilon_e^{TM}(k_q)\hat{\mathbf{z}}\hat{\mathbf{z}}. \tag{S76}$$

Use of this symmetry enables us to simplify the left-side of Eq. (S16):

$$\phi_p \mathbf{L}_p^{(q)} \cdot [\mathbf{L}_e(\mathbf{k}_q)]^{-1} \cdot \phi_p \mathbf{L}_p^{(q)} = \frac{[\phi_p(2\varepsilon_q)\beta_{pq}^{(2D)}]^2}{2\varepsilon_q} \frac{\varepsilon_e^{TE}(k_q) + \varepsilon_q}{\varepsilon_e^{TE}(k_q) - \varepsilon_q} (\mathbf{I} - \hat{\mathbf{z}}\hat{\mathbf{z}}) + [\phi_p(\varepsilon_p + \varepsilon_q)\beta_{pq}^{(2D)}]^2 \frac{1}{\varepsilon_e^{TM}(k_q) - \varepsilon_q} \hat{\mathbf{z}}\hat{\mathbf{z}}, \quad (\text{S77})$$

which gives two *non-scaled* multiple-scattering approximations for TE and TM polarizations, respectively:

$$\frac{[\phi_p(2\varepsilon_q)\beta_{pq}^{(2D)}]^2}{2\varepsilon_q} \frac{\varepsilon_e^{TE}(k_q) + \varepsilon_q}{\varepsilon_e^{TE}(k_q) - \varepsilon_q} = \phi_p[2\varepsilon_q\beta_{pq}^{(2D)}] - A_2^{TE}(k_q; \varepsilon_q) [2\varepsilon_q\beta_{pq}^{(2D)}]^2 - A_3^{TE}(k_q; \varepsilon_q) [2\varepsilon_q\beta_{pq}^{(2D)}]^3 \\ - \dots - A_n^{TE}(k_q; \varepsilon_q) [2\varepsilon_q\beta_{pq}^{(2D)}]^n, \quad (\text{S78})$$

$$\frac{[\phi_p(\varepsilon_p + \varepsilon_q)\beta_{pq}^{(2D)}]^2}{\varepsilon_e^{TM}(k_q) - \varepsilon_q} = \phi_p[(\varepsilon_p + \varepsilon_q)\beta_{pq}^{(2D)}] - A_2^{TM}(k_q; \varepsilon_q) [(\varepsilon_p + \varepsilon_q)\beta_{pq}^{(2D)}]^2 - A_3^{TM}(k_q; \varepsilon_q) [(\varepsilon_p + \varepsilon_q)\beta_{pq}^{(2D)}]^3 \\ - \dots - A_n^{TM}(k_q; \varepsilon_q) [(\varepsilon_p + \varepsilon_q)\beta_{pq}^{(2D)}]^n, \quad (\text{S79})$$

150 where  $A_n^{TE}(k_q; \varepsilon_q) \equiv [2\varepsilon_q\beta_{pq}^{(2D)}]^{-n}(\mathbf{I} - \hat{\mathbf{z}}\hat{\mathbf{z}}) : \mathcal{A}_n^{(p)}(k_q) / 2$  and  $A_n^{TM}(k_q; \varepsilon_q) \equiv [(\varepsilon_p + \varepsilon_q)\beta_{pq}^{(2D)}]^{-n}(\hat{\mathbf{z}}\hat{\mathbf{z}}) :$   
 151  $\mathcal{A}_n^{(p)}(k_q)$ . We call Eq. (S78) and Eq. (S79) *non-scaled* strong-contrast approximations that take  
 152 either phase 1 or 2 as the reference phase, i.e.,  $q = 1, 2$ . In Sec. 4, we derive the scaled variants of  
 153 Eq. (S78) and Eq. (S79) by renormalizing them with the optimal reference phase.

We now obtain the second-order coefficients  $A_2^{TE}(k_q; \varepsilon_q)$  and  $A_2^{TM}(k_q; \varepsilon_q)$  from a simplified expression of Eq. (S74):

$$\mathcal{A}_2^{(p)}(k_q) = \frac{[\beta_{pq}^{(2D)}]^2}{2\varepsilon_q} \frac{1}{(2\pi)^2} \int_{\mathbb{R}^2} \frac{d\mathbf{q}_\perp}{|k_q\hat{\mathbf{y}} + \mathbf{q}_\perp|^2 - k_q^2} \left\{ (2\varepsilon_q)^2 [ (|k_q\hat{\mathbf{y}} + \mathbf{q}_\perp|^2 + k_q^2)(\mathbf{I} - \hat{\mathbf{z}}\hat{\mathbf{z}}) - 2(k_q\hat{\mathbf{y}} + \mathbf{q}_\perp)(k_q\hat{\mathbf{y}} + \mathbf{q}_\perp) \right. \\ \left. + (\varepsilon_q + \varepsilon_p)^2 2k_q^2 \hat{\mathbf{z}}\hat{\mathbf{z}} \right\} \tilde{\chi}_v(q_\perp), \quad (\text{S80})$$

where we have used the normal incidence condition. Using Eq. (S80), we then obtain

$$A_2^{TE}(k_q; \varepsilon_q) \equiv [2\varepsilon_q\beta_{pq}^{(2D)}]^{-2} \frac{\mathbf{I} - \hat{\mathbf{z}}\hat{\mathbf{z}}}{2} : \mathcal{A}_2^{(p)}(k_q) \\ = \frac{1}{2\varepsilon_q} \frac{1}{(2\pi)^2} \int_{\mathbb{R}^2} \frac{d\mathbf{q}_\perp}{|k_q\hat{\mathbf{y}} + \mathbf{q}_\perp|^2 - k_q^2} [ (|k_q\hat{\mathbf{y}} + \mathbf{q}_\perp|^2 + k_q^2) - |k_q\hat{\mathbf{y}} + \mathbf{q}_\perp|^2 ] \tilde{\chi}_v(q_\perp) \\ = \frac{k_q^2}{2\varepsilon_q} \frac{1}{(2\pi)^2} \int_{\mathbb{R}^2} \frac{d\mathbf{q}_\perp}{|k_q\hat{\mathbf{y}} + \mathbf{q}_\perp|^2 - k_q^2} \tilde{\chi}_v(q_\perp), \quad (\text{S81})$$

$$A_2^{TM}(k_q; \varepsilon_q) \equiv [(\varepsilon_p + \varepsilon_q)\beta_{pq}^{(2D)}]^{-2} (\hat{\mathbf{z}}\hat{\mathbf{z}}) : \mathcal{A}_2^{(p)}(k_q) = \frac{k_q^2}{\varepsilon_q} \frac{1}{(2\pi)^2} \int_{\mathbb{R}^2} \frac{d\mathbf{q}_\perp}{|k_q\hat{\mathbf{y}} + \mathbf{q}_\perp|^2 - k_q^2} \tilde{\chi}_v(q_\perp), \quad (\text{S82})$$

where these two coefficients are related to the nonlocal attenuation function  $F^{(2D)}(k)$  for 2D statistically isotropic media [4] as follows:

$$F^{(2D)}(k) = -\frac{4\varepsilon_q}{\pi} A_2^{TE}(k; \varepsilon_q) = -\frac{2\varepsilon_q}{\pi} A_2^{TM}(k; \varepsilon_q) \\ = \frac{-2}{\pi} \left\{ \frac{k_q^2}{\pi^2} \int_0^{\pi/2} d\phi \left[ \text{p.v.} \int_0^\infty dq \frac{2q \tilde{\chi}_v(q)}{q^2 - (2k_q \cos \phi)^2} \right] + i \frac{k_q^2}{\pi} \int_0^{\pi/2} \tilde{\chi}_v(2k_q \cos \phi) d\phi \right\} \quad (\text{S83})$$

We obtain the expressions for the third-order coefficients  $A_3^{TE}(k_q; \varepsilon_q)$  and  $A_3^{TM}(k_q; \varepsilon_q)$ . Taking  $\mathbf{X} = k_q \hat{\mathbf{y}} + \mathbf{q}_1$  and  $\mathbf{Y} = k_q \hat{\mathbf{y}} + \mathbf{q}_2$ , we reduce the third-order tensor [Eq. (S75)] as

$$\begin{aligned} \mathcal{A}_3^{(p)}(\mathbf{k}_q) = & \left( \frac{-1}{\phi_p} \right) \frac{[\beta_{pq}^{(2D)}]^3}{(2\varepsilon_q)^2} \frac{1}{(2\pi)^4} \int_{\mathbb{R}^2} d\mathbf{q}_1 d\mathbf{q}_2 \frac{\tilde{\Delta}_3^{(p)}(-\mathbf{q}_1, -\mathbf{q}_2)}{|\mathbf{k}_q + \mathbf{q}_1|^2 - k_q^2} \frac{1}{|\mathbf{k}_q + \mathbf{q}_2|^2 - k_q^2} \times \\ & \left( (2\varepsilon_q)^3 \{ (|\mathbf{k}_q \hat{\mathbf{y}} + \mathbf{q}_1|^2 + k_q^2) [ (|\mathbf{k}_q \hat{\mathbf{y}} + \mathbf{q}_2|^2 + k_q^2) (\mathbf{I} - \hat{\mathbf{z}}\hat{\mathbf{z}}) - 2(k_q \hat{\mathbf{y}} + \mathbf{q}_2)(k_q \hat{\mathbf{y}} + \mathbf{q}_2) ] \right. \\ & \quad \left. - 2(|\mathbf{k}_q \hat{\mathbf{y}} + \mathbf{q}_2|^2 + k_q^2)(k_q \hat{\mathbf{y}} + \mathbf{q}_1)(k_q \hat{\mathbf{y}} + \mathbf{q}_1) + 4[(k_q \hat{\mathbf{y}} + \mathbf{q}_1) \cdot (k_q \hat{\mathbf{y}} + \mathbf{q}_2)](k_q \hat{\mathbf{y}} + \mathbf{q}_1)(k_q \hat{\mathbf{y}} + \mathbf{q}_2) \right\} \\ & \quad + (\varepsilon_p + \varepsilon_q)^3 (2k_q^2)^2 \hat{\mathbf{z}}\hat{\mathbf{z}} \Big). \end{aligned} \quad (\text{S84})$$

From this expression, we obtain the following two third-order coefficients:

$$\begin{aligned} A_3^{TE}(k_q; \varepsilon_q) & \equiv [2\varepsilon_q \beta_{pq}^{(2D)}]^{-3} \frac{\mathbf{I} - \hat{\mathbf{z}}\hat{\mathbf{z}}}{2} : \mathcal{A}_3^{(p)}(k_q) \\ & = \left( \frac{-1}{\phi_p} \right) \frac{1}{(2\varepsilon_q)^2} \frac{1}{(2\pi)^4} \int_{\mathbb{R}^2} d\mathbf{q}_1 d\mathbf{q}_2 \frac{\tilde{\Delta}_3^{(p)}(\mathbf{q}_1, \mathbf{q}_2)}{|\mathbf{k}_q + \mathbf{q}_1|^2 - k_q^2} \frac{1}{|\mathbf{k}_q + \mathbf{q}_2|^2 - k_q^2} \\ & \quad \times \{ (|\mathbf{k}_q \hat{\mathbf{y}} + \mathbf{q}_1|^2 + k_q^2) [ (|\mathbf{k}_q \hat{\mathbf{y}} + \mathbf{q}_2|^2 + k_q^2) - |\mathbf{k}_q \hat{\mathbf{y}} + \mathbf{q}_2|^2 ] - (|\mathbf{k}_q \hat{\mathbf{y}} + \mathbf{q}_2|^2 + k_q^2) |\mathbf{k}_q \hat{\mathbf{y}} + \mathbf{q}_1|^2 + 2[(\mathbf{k}_q \hat{\mathbf{y}} + \mathbf{q}_1) \cdot (\mathbf{k}_q \hat{\mathbf{y}} + \mathbf{q}_2)]^2 \} \\ & = \left( \frac{-1}{\phi_p} \right) \frac{1}{(2\varepsilon_q)^2} \frac{1}{(2\pi)^4} \int_{\mathbb{R}^2} d\mathbf{q}_1 d\mathbf{q}_2 \frac{[(k_q^2)^2 - |\mathbf{k}_q \hat{\mathbf{y}} + \mathbf{q}_1|^2 |\mathbf{k}_q \hat{\mathbf{y}} + \mathbf{q}_2|^2 + 2[(\mathbf{k}_q \hat{\mathbf{y}} + \mathbf{q}_1) \cdot (\mathbf{k}_q \hat{\mathbf{y}} + \mathbf{q}_2)]^2]}{[|\mathbf{k}_q + \mathbf{q}_1|^2 - k_q^2][|\mathbf{k}_q + \mathbf{q}_2|^2 - k_q^2]} \\ & \quad \times \tilde{\Delta}_3^{(p)}(\mathbf{q}_1, \mathbf{q}_2), \end{aligned} \quad (\text{S85})$$

$$\begin{aligned} A_3^{TM}(k_q; \varepsilon_q) & \equiv [(\varepsilon_p + \varepsilon_q) \beta_{pq}^{(2D)}]^{-3} (\hat{\mathbf{z}}\hat{\mathbf{z}}) : \mathcal{A}_3^{(p)}(k_q) \\ & = \left( \frac{-1}{\phi_p} \right) \frac{(k_q^2)^2}{(\varepsilon_q)^2} \frac{1}{(2\pi)^4} \int_{\mathbb{R}^2} d\mathbf{q}_1 d\mathbf{q}_2 \frac{\tilde{\Delta}_3^{(p)}(\mathbf{q}_1, \mathbf{q}_2)}{|\mathbf{k}_q + \mathbf{q}_1|^2 - k_q^2} \frac{1}{|\mathbf{k}_q + \mathbf{q}_2|^2 - k_q^2}, \end{aligned} \quad (\text{S86})$$

154 The second- and third-order coefficients for TE [Eq. (S81) and Eq. (S85)] and TM [Eq. (S82) and  
155 Eq. (S86)] polarizations are complex-valued, implying that the media are effectively lossy for both  
156 polarizations due to scatterings.

In the static limit (i.e.,  $k \rightarrow 0^+$ ), three coefficients  $A_2^{TE}(k; \varepsilon_q)$ ,  $A_2^{TM}(k; \varepsilon_q)$ ,  $A_3^{TM}(k; \varepsilon_q)$  [see Eq. (S81), Eq. (S82), and Eq. (S86)] vanish. By contrast, the third-order coefficient for the TE polarization converges to

$$\begin{aligned} A_3^{TE}(0; \varepsilon_q) & = \left( \frac{-1}{\phi_p} \right) \frac{1}{(2\varepsilon_q)^2} \frac{1}{(2\pi)^4} \int_{\mathbb{R}^2} d\mathbf{q}_1 d\mathbf{q}_2 \frac{[2(\mathbf{q}_1 \cdot \mathbf{q}_2)^2 - q_1^2 q_2^2]}{q_1^2 q_2^2} \tilde{\Delta}_3^{(p)}(-\mathbf{q}_1, -\mathbf{q}_2) \\ & = \frac{-1/\phi_p}{(2\varepsilon_q)^2} \left[ \frac{2}{(2\pi)^4} \int_{\mathbb{R}^2} d\mathbf{q}_1 d\mathbf{q}_2 \frac{(\mathbf{q}_1 \cdot \mathbf{q}_2)^2}{q_1^2 q_2^2} \tilde{\Delta}_3^{(p)}(-\mathbf{q}_1, -\mathbf{q}_2) - \frac{1}{(2\pi)^4} \int_{\mathbb{R}^2} d\mathbf{q}_1 d\mathbf{q}_2 \tilde{\Delta}_3^{(p)}(-\mathbf{q}_1, -\mathbf{q}_2) \right] \\ & = \frac{-1/\phi_p}{(2\varepsilon_q)^2} \left[ -\phi_p^2 \phi_q \zeta_p - \Delta_3^{(p)}(\mathbf{r} = \mathbf{0}, \mathbf{s} = \mathbf{0}) \right] = \frac{\phi_p \phi_q}{(2\varepsilon_q)^2} \zeta_p, \end{aligned} \quad (\text{S87})$$

where  $\zeta_p$  is the three-point parameter that lies in the closed interval  $[0, 1]$  [1]. Consequently, for TE polarization, the third-order approximation [Eq. (S78) where  $n = 3$ ] recovers the static strong-contrast approximations for  $d = 2$ :

$$\varepsilon_e^{TE}(0) = \varepsilon_q \frac{\phi_p(1 + \phi_p \beta_{pq}^{(2D)}) - (1 - \phi_p) \zeta_p [\beta_{pq}^{(2D)}]^2}{\phi_p(1 - \phi_p \beta_{pq}^{(2D)}) - (1 - \phi_p) \zeta_p [\beta_{pq}^{(2D)}]^2}. \quad (\text{S88})$$

For TM polarization, the third-order approximation [Eq. (S79), where  $n = 3$ ] converges to the arithmetic mean of the local dielectric constant:

$$\varepsilon_e^{TM}(0) = \langle \varepsilon \rangle = \phi_p \varepsilon_p + \phi_q \varepsilon_q. \quad (\text{S89})$$

#### D. Perfect Transparency at the Three-Point Level

In section 4 of the main text, we analytically show that the finite perfect transparency interval [Eq. (26) of the main text] for TM polarization in transversely isotropic stealthy hyperuniform systems (or, equivalently, 2D stealthy hyperuniform systems) is exact through the third-order terms. There, we outline the proof of a perfect transparency condition related to the third-order term  $A_3^{TM}$ ; see Eq. (37) of the main text. Here, we provide a detailed proof of Eq. (37) of the main text.

Without losing generality, we can rewrite the third-order condition [Eq. (37)] as follows:

$$\text{Im}[A_3^{TM}(k; 1)] = 0, \quad (k < K/2). \quad (\text{S90})$$

As in Sec. S2D, we substitute the explicit expression of  $\tilde{\Delta}_3^{(p)}(\mathbf{q}_1, \mathbf{q}_2)$ , Eq. (S25), into the Fourier representation of  $A_3^{TM}$  [Eq. (S86)] and then decompose  $A_3^{TM}$  into three terms:

$$\begin{aligned} A_3^{TM}(k; 1) &= \frac{-1}{\phi_p} \frac{k^4}{(2\pi)^4} \int_{\mathbb{R}^2} d\mathbf{q}_1 \int_{\mathbb{R}^2} d\mathbf{q}_2 \frac{1}{|k\hat{\mathbf{y}} + \mathbf{q}_1|^2 - k^2} \frac{1}{|k\hat{\mathbf{y}} + \mathbf{q}_2|^2 - k^2} \\ &\quad \times \left[ \tilde{\chi}_v(q_1) \tilde{\chi}_v(q_2) - \phi_p^2 (2\pi)^2 \delta(\mathbf{q}_1 - \mathbf{q}_2) \tilde{\chi}_v(q_2) - \phi_p \langle \tilde{\mathcal{J}}^{(p)}(-\mathbf{q}_1) \tilde{\mathcal{J}}^{(p)}(\mathbf{q}_1 - \mathbf{q}_2) \tilde{\mathcal{J}}^{(p)}(\mathbf{q}_2) \rangle \right] \\ &= \frac{-1}{\phi_p} \frac{k^4}{(2\pi)^4} [C_1^{TM}(k) - \phi_p^2 (2\pi)^2 C_2^{TM}(k) - \phi_p C_3^{TM}(k)], \end{aligned} \quad (\text{S91})$$

where  $C_1^{TM}(k)$  and  $C_2^{TM}(k)$  depend on the two-point statistics, whereas  $C_3^{TM}(k)$  depends on the three-point statistics:

$$C_1^{TM}(k) \equiv \left[ -\frac{2\pi^3}{k^2} F^{(2D)}(k) \right]^2, \quad (\text{S92})$$

$$C_2^{TM}(k) \equiv \int_{\mathbb{R}^2} d\mathbf{q}_1 \left[ \frac{1}{|k\hat{\mathbf{y}} + \mathbf{q}_1|^2 - k^2} \right]^2 \tilde{\chi}_v(q_1), \quad (\text{S93})$$

$$C_3^{TM}(k) \equiv \int_{\mathbb{R}^2} d\mathbf{q}_1 \int_{\mathbb{R}^2} d\mathbf{q}_2 \frac{1}{|k\hat{\mathbf{y}} + \mathbf{q}_1|^2 - k^2} \frac{1}{|k\hat{\mathbf{y}} + \mathbf{q}_2|^2 - k^2} \langle \tilde{\mathcal{J}}^{(p)}(\mathbf{q}_1) \tilde{\mathcal{J}}^{(p)}(-\mathbf{q}_1 + \mathbf{q}_2) \tilde{\mathcal{J}}^{(p)}(-\mathbf{q}_2) \rangle, \quad (\text{S94})$$

which are the 2D counterparts of Eq. (S49)-Eq. (S51). We now prove Eq. (S90) by showing that for  $n = 1, 2, 3$ ,

$$\text{Im}[C_n^{TM}(k)] = 0 \quad (k < K/2). \quad (\text{S95})$$

The proof of Eq. (S95) is analogous to what we did in Sec. S2D. Specifically, we utilize the three general properties of  $\tilde{\mathcal{J}}^{(p)}(\mathbf{k})$  for 2D disordered stealthy hyperuniform two-phase media:

$$\text{Stealthy hyperuniform condition: } \left| \tilde{\mathcal{J}}^{(p)}(\mathbf{k}) \right| = 0, \quad \text{for } 0 \leq |\mathbf{k}| < K, \quad (\text{S96})$$

$$\text{No Bragg peaks: } \left| \tilde{\mathcal{J}}^{(p)}(\mathbf{k}) \right| < C, \quad \text{for any } \mathbf{k}, \quad (\text{S97})$$

$$\text{Large-}k \text{ scaling from Eq. (S3): } \left| \tilde{\mathcal{J}}^{(p)}(\mathbf{k}) \right| \leq \frac{C'}{|\mathbf{k}|^{3/2}}, \quad \text{for } Q \leq |\mathbf{k}|, \quad (\text{S98})$$

where  $C'$  and  $C$  are finite positive numbers, and  $Q$  is a large wave number much greater than  $K$ .

One can immediately see that Eq. (S95) is true for  $n = 1$  because  $\text{Im}[F^{(2D)}(k)] = 0$  for  $k < K/2$  as shown in Eq. (S83). We then prove Eq. (S95) for  $n = 2$  by showing that the integral involving in Eq. (S93) is real-valued for  $k < K/2$  because its integrand is real-valued and absolutely integrable. The integrand in Eq. (S93) is real-valued and nonnegative except at singularities because it is the product of the spectral density  $\tilde{\chi}_v(q_1)$  and the square of Green's function [i.e.,  $(|k\hat{\mathbf{y}} + \mathbf{q}_1|^2 - k^2)^{-2}$ ] for any  $k$ . For  $k < K/2$ , this integrand has no singularity because the stealthy hyperuniform condition [Eq. (S96)] completely removes the singularities that the Green's function can arise, similar to the case of  $k_* < K/2$  in Fig. 2(a) of the main text. Furthermore, due to the properties of  $\tilde{\chi}_v(k)$  [Eq. (S97) and Eq. (S98)], this nonnegative integrand of Eq. (S93) is bounded from above and

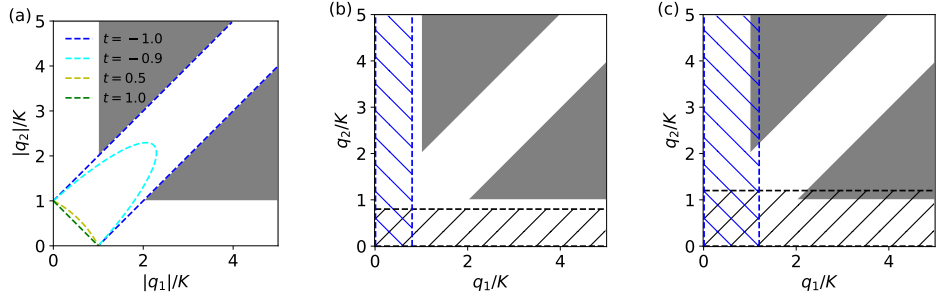

**Fig. S1.** (a) The exclusion region (shown in white) of the three-point function  $\langle \tilde{\mathcal{J}}^{(p)}(\mathbf{q}_1) \tilde{\mathcal{J}}^{(p)}(-\mathbf{q}_1 + \mathbf{q}_2) \tilde{\mathcal{J}}^{(p)}(-\mathbf{q}_2) \rangle$  in terms of a pair of wave numbers  $(q_1, q_2)$  for a transversely isotropic stealthy hyperuniform model. The diagonal white strip depicts the region where  $\tilde{\mathcal{J}}^{(p)}(-\mathbf{q}_1 + \mathbf{q}_2) = 0$ . The dashed lines depict the edges of the exclusion regions for  $\tilde{\mathcal{J}}^{(p)}(-\mathbf{q}_1 + \mathbf{q}_2)$  at given values of  $\cos \theta$ , where  $\theta$  is the angle between  $-\mathbf{q}_1$  and  $\mathbf{q}_2$ . (b,c) Loci of singularities (shown in the hatched regions) of the integrand involving  $C_3^{TM}(k)$ , Eq. (S94), in two cases: (b)  $k < K/2$  and (c)  $k > K/2$ . The white region depicts the exclusion region at the three-point level constructed in (a). When  $k < K/2$ , all singularities lie inside the exclusion region.

174 decays rapidly as  $|\mathbf{q}_1|$  increases. Therefore, for  $k < K/2$ , the real-valued integrand of Eq. (S93) is  
 175 absolutely integrable, leading to  $\text{Im}[C_2^{TM}(k)] = 0$ .

176 We now prove Eq. (S95) for  $n = 3$ . Similar to the proof of Eq. (S52) for  $n = 3$ , the crucial part of  
 177 this proof is to show that for  $k < K/2$ , the absolute value of the integrand in Eq. (S94) is integrable  
 178 (i.e., absolutely integrable), and thus the value of  $C_3^{TM}(k)$  is independent of the integration order  
 179 due to the Fubini-Tonelli theorem [16]. Once we show the interchangeability of integration order,  
 180 as in the proof of  $\text{Im}[C_3^{\perp}(k)] = 0$  for  $k < K/2$  (see Sec. S2D), we can immediately show that  
 181  $C_3^{TM}(k)^* = C_3^{TM}(k)$  or, equivalently, Eq. (S95) for  $n = 3$  is true.

182 Using Eq. (S96), we first find the exclusion region at the three-point level in terms of wave  
 183 numbers  $q_1$  and  $q_2$ , in which the three-point function  $\langle \tilde{\mathcal{J}}^{(p)}(\mathbf{q}_1) \tilde{\mathcal{J}}^{(p)}(-\mathbf{q}_1 + \mathbf{q}_2) \tilde{\mathcal{J}}^{(p)}(-\mathbf{q}_2) \rangle = 0$ .  
 184 As shown in Fig. S1(a), this exclusion region is found from the union of three conditions:  $0 \leq$   
 185  $q_1 < K$ ,  $0 \leq q_2 < K$ , or  $0 \leq |-\mathbf{q}_1 + \mathbf{q}_2|^2 = q_1^2 + q_2^2 + 2tq_1q_2 < K^2$ , where  $-1 \leq t (\equiv \cos \theta) \leq 1$ ,  
 186 and  $\theta$  is the angle between  $-\mathbf{q}_1$  and  $\mathbf{q}_2$ . By contrast, all singularities that the Green's functions  
 187 in Eq. (S94) have lie along two circles [i.e.,  $|\mathbf{q}_1 + k\hat{\mathbf{y}}| = k$  and  $|\mathbf{q}_2 + k\hat{\mathbf{y}}| = k$ ], which simplify to  
 188  $0 \leq q_1 < 2k$  and  $0 \leq q_2 < 2k$ , respectively. Figure S1(b,c) demonstrates that only if  $k < K/2$ ,  
 189 all singularities of the Green's functions (shown in the hatched regions) lie inside the exclusion  
 190 region. Thus, the integrand in Eq. (S94) has no singularity, implying that its value is bounded  
 191 everywhere if  $k < K/2$ .

Now let us show that the integrand in  $C_3^{TM}(k)$  is absolutely integrable when  $k < K/2$ . We  
 simplify the absolute value of this integrand as follows:

$$\begin{aligned}
 & \left| \frac{1}{|k\hat{\mathbf{y}} + \mathbf{q}_1|^2 - k^2} \frac{1}{|k\hat{\mathbf{y}} + \mathbf{q}_2|^2 - k^2} \langle \tilde{\mathcal{J}}^{(p)}(\mathbf{q}_1) \tilde{\mathcal{J}}^{(p)}(-\mathbf{q}_1 + \mathbf{q}_2) \tilde{\mathcal{J}}^{(p)}(-\mathbf{q}_2) \rangle \right| \\
 & \leq \left| \frac{1}{|k\hat{\mathbf{y}} + \mathbf{q}_1|^2 - k^2} \frac{1}{|k\hat{\mathbf{y}} + \mathbf{q}_2|^2 - k^2} \right| \left| \langle \tilde{\mathcal{J}}^{(p)}(\mathbf{q}_1) \tilde{\mathcal{J}}^{(p)}(-\mathbf{q}_1 + \mathbf{q}_2) \tilde{\mathcal{J}}^{(p)}(-\mathbf{q}_2) \rangle \right| \\
 & \leq \left| \frac{1}{|k\hat{\mathbf{y}} + \mathbf{q}_1|^2 - k^2} \frac{1}{|k\hat{\mathbf{y}} + \mathbf{q}_2|^2 - k^2} \right| C \left| \langle \tilde{\mathcal{J}}^{(p)}(\mathbf{q}_1) \tilde{\mathcal{J}}^{(p)}(-\mathbf{q}_2) \rangle \right| = C \left\langle \left| \frac{\tilde{\mathcal{J}}^{(p)}(\mathbf{q}_1)}{|k\hat{\mathbf{y}} + \mathbf{q}_1|^2 - k^2} \right| \left| \frac{\tilde{\mathcal{J}}^{(p)}(-\mathbf{q}_2)}{|k\hat{\mathbf{y}} + \mathbf{q}_2|^2 - k^2} \right| \right\rangle, \tag{S99}
 \end{aligned}$$

where we have used Eq. (S97). The integral of Eq. (S99) is

$$\begin{aligned} & \int_{\mathbb{R}^2} d\mathbf{q}_1 \int_{\mathbb{R}^2} d\mathbf{q}_2 \left\langle \left| \frac{\tilde{\mathcal{J}}^{(p)}(\mathbf{q}_1)}{|k\hat{\mathbf{y}} + \mathbf{q}_1|^2 - k^2} \right| \left| \frac{\tilde{\mathcal{J}}^{(p)}(-\mathbf{q}_2)}{|k\hat{\mathbf{y}} + \mathbf{q}_2|^2 - k^2} \right| \right\rangle = \left\langle \int_{\mathbb{R}^2} d\mathbf{q}_1 \left| \frac{\tilde{\mathcal{J}}^{(p)}(\mathbf{q}_1)}{|k\hat{\mathbf{y}} + \mathbf{q}_1|^2 - k^2} \right| \int_{\mathbb{R}^2} d\mathbf{q}_2 \left| \frac{\tilde{\mathcal{J}}^{(p)}(-\mathbf{q}_2)}{|k\hat{\mathbf{y}} + \mathbf{q}_2|^2 - k^2} \right| \right\rangle \\ &= \left\langle \left\{ \int_{0 \leq |\mathbf{q}_1| < K} d\mathbf{q}_1 \left| \frac{\tilde{\mathcal{J}}^{(p)}(\mathbf{q}_1)}{|k\hat{\mathbf{y}} + \mathbf{q}_1|^2 - k^2} \right| + \int_{K \leq |\mathbf{q}_1| < Q} d\mathbf{q}_1 \left| \frac{\tilde{\mathcal{J}}^{(p)}(\mathbf{q}_1)}{|k\hat{\mathbf{y}} + \mathbf{q}_1|^2 - k^2} \right| + \int_{Q \leq |\mathbf{q}_1|} d\mathbf{q}_1 \left| \frac{\tilde{\mathcal{J}}^{(p)}(\mathbf{q}_1)}{|k\hat{\mathbf{y}} + \mathbf{q}_1|^2 - k^2} \right| \right\}^2 \right\rangle. \end{aligned} \quad (\text{S100})$$

For a moment, we focus on the three integrals appearing in Eq. (S100). The first integral is exactly zero because of Eq. (S96):

$$\int_{0 \leq |\mathbf{q}_1| < K} d\mathbf{q}_1 \left| \frac{\tilde{\mathcal{J}}^{(p)}(\mathbf{q}_1)}{|k\hat{\mathbf{y}} + \mathbf{q}_1|^2 - k^2} \right| = 0. \quad (\text{S101})$$

Using Eq. (S97), we show that the second integral is bounded above:

$$\begin{aligned} \int_{K \leq |\mathbf{q}_1| < Q} d\mathbf{q}_1 \left| \frac{\tilde{\mathcal{J}}^{(p)}(\mathbf{q}_1)}{|k\hat{\mathbf{y}} + \mathbf{q}_1|^2 - k^2} \right| &\leq C \int_{K \leq |\mathbf{q}_1| < Q} d\mathbf{q}_1 \left| \frac{1}{|k\hat{\mathbf{y}} + \mathbf{q}_1|^2 - k^2} \right| \leq \frac{C}{K(K-2k)} \int_{K \leq |\mathbf{q}_1| < Q} d\mathbf{q}_1 \\ &= \frac{C\pi(Q^2 - K^2)}{K(K-2k)}. \end{aligned} \quad (\text{S102})$$

The third integral in Eq. (S100) is also bounded above:

$$\begin{aligned} \int_{Q \leq |\mathbf{q}_1|} d\mathbf{q}_1 \left| \frac{\tilde{\mathcal{J}}^{(p)}(\mathbf{q}_1)}{|k\hat{\mathbf{y}} + \mathbf{q}_1|^2 - k^2} \right| &= C' \int_{Q \leq |\mathbf{q}_1|} d\mathbf{q}_1 \left| \frac{q_1^{-3/2}}{|k\hat{\mathbf{y}} + \mathbf{q}_1|^2 - k^2} \right| = C' \int_Q^\infty dq_1 q_1 \int_0^{2\pi} d\phi \frac{q_1^{-3/2}}{q_1^2 [1 + (2k/q_1) \cos \phi]} \\ &= C' \int_Q^\infty dq_1 \frac{1}{q_1^{5/2}} \frac{2\pi}{\sqrt{1 - (2k/q_1)^2}} \leq C' \int_Q^\infty dq_1 \frac{1}{q_1^{5/2}} \frac{2\pi}{\sqrt{1 - (2k/Q)^2}} \\ &= \frac{4\pi C'}{3} \frac{1}{Q^{3/2} \sqrt{1 - (2k/Q)^2}}, \end{aligned} \quad (\text{S103})$$

where we have used Eq. (S98) and  $\int_0^{2\pi} dx (1 + c \cos x)^{-1} = 2\pi / \sqrt{1 - c^2}$  if  $|c| < 1$ . Combining Eq. (S99)-Eq. (S103) together, we can show that the integrand of Eq. (S94) is indeed absolutely integrable for  $k < K/2$ :

$$\begin{aligned} & \int_{\mathbb{R}^2} d\mathbf{q}_1 \int_{\mathbb{R}^2} d\mathbf{q}_2 \left| \frac{1}{|k\hat{\mathbf{y}} + \mathbf{q}_1|^2 - k^2} \frac{1}{|k\hat{\mathbf{y}} + \mathbf{q}_2|^2 - k^2} \langle \tilde{\mathcal{J}}^{(p)}(\mathbf{q}_1) \tilde{\mathcal{J}}^{(p)}(-\mathbf{q}_1 + \mathbf{q}_2) \tilde{\mathcal{J}}^{(p)}(-\mathbf{q}_2) \rangle \right| \\ &\leq C \left\{ \frac{C\pi(Q^2 - K^2)}{K(K-2k)} + \frac{4\pi C'}{3} \frac{1}{Q^{3/2} \sqrt{1 - (2k/Q)^2}} \right\}^2. \end{aligned} \quad (\text{S104})$$

#### 192 4. SCALED APPROXIMATIONS

It is important to note that while the full strong-contrast series [Eq. (S6)] gives exact effective dielectric constant tensor independent of the dielectric constant tensor  $\epsilon_q$  of the reference phase, the value of  $\epsilon_q$  does determine the convergence rate of the series. This implies that the choice of the reference phase can improve or worsen the accuracy of the lower-order truncations (or approximations) of the series for  $\epsilon_e(\mathbf{k}_q)$ . The optimal reference phase (its dielectric constant denoted by  $\epsilon_*$ ) for the fastest convergence meets the following condition:

$$\langle L^{(*)}(\mathbf{x}) \rangle \equiv L_1^{(*)} \phi_1 + L_2^{(*)} \phi_2 = 0, \quad (\text{S105})$$

193 because the effective dynamic dielectric constant  $\epsilon_e(\mathbf{k}_q)$  of a composite is very close (but not  
194 identical) to the dielectric constant  $\epsilon_*$  of the such a reference phase ( $q = *$ ), and thus scattering  
195 becomes very weak through all orders so that the series converges very rapidly [8, 18]. In what  
196 follows, we derive the renormalized strong-contrast formulas for the layered and transversely  
197 isotropic media.

For layered media, due to the azimuthal symmetry,  $\varepsilon_*$  of the optimal reference phase should have the form:  $\varepsilon_* = a(\mathbf{I} - \hat{\mathbf{z}}\hat{\mathbf{z}}) + b\hat{\mathbf{z}}\hat{\mathbf{z}}$ . Then, considering the disk-like exclusion volume, one can find that the expression for the dyadic source term as  $\mathbf{D}^{(*)} = b^{-1}\hat{\mathbf{z}}\hat{\mathbf{z}}$ . Substituting these two expressions to Eq. (S105) and solving them with respect to  $a$  and  $b$  yield

$$\varepsilon_* = \langle \varepsilon \rangle (\mathbf{I} - \hat{\mathbf{z}}\hat{\mathbf{z}}) + \langle 1/\varepsilon \rangle^{-1} \hat{\mathbf{z}}\hat{\mathbf{z}} = \varepsilon_e^\perp(0) (\mathbf{I} - \hat{\mathbf{z}}\hat{\mathbf{z}}) + \varepsilon_e^z(0) \hat{\mathbf{z}}\hat{\mathbf{z}}, \quad (\text{S106})$$

where  $\langle \varepsilon \rangle \equiv \phi_1 \varepsilon_1 + \phi_2 \varepsilon_2$  and  $\langle 1/\varepsilon \rangle \equiv \phi_1/\varepsilon_1 + \phi_2/\varepsilon_2$ . Note that Eq. (S106) is identical to the effective static dielectric constant of the layered media. Application of such a renormalization to the strong-contrast approximation [Eq. (S45) at the three-point level] is equivalent to replacing the Green's function  $\tilde{\mathbf{H}}^{(q)}(\mathbf{k})$  in the matrix phase  $q$  in Eq. (S38) with  $\tilde{\mathbf{H}}^{(*)}(\mathbf{k})$  in the reference phase with  $\varepsilon_*$  given by Eq. (S106) and yields the *scaled* (or renormalized) strong-contrast approximation for disordered layered media [15]:

$$\varepsilon_e^\perp(k_q) = \varepsilon_q \left[ 1 + \frac{\phi_p^2 (\varepsilon_p/\varepsilon_q) \beta_{pq}^{(1D)}}{\phi_p - (\varepsilon_p \beta_{pq}^{(1D)}) A_2^\perp(k_*; \langle \varepsilon \rangle) - (\varepsilon_p \beta_{pq}^{(1D)})^2 A_3^\perp(k_*; \langle \varepsilon \rangle)} \right], \quad (\text{S107})$$

198 where  $k_* = k_q \sqrt{\langle \varepsilon \rangle / \varepsilon_q}$  is the wave number for the transverse polarization in the optimal reference  
199 phase.

For transversely isotropic media, due to the azimuthal symmetry,  $\varepsilon_I$  of the optimal reference phase also has the form:  $\varepsilon_* = a(\mathbf{I} - \hat{\mathbf{z}}\hat{\mathbf{z}}) + b\hat{\mathbf{z}}\hat{\mathbf{z}}$ . Then, considering the needle-like exclusion volume, one can find that the expression for the dyadic source term as  $\mathbf{D}^{(*)} = (2a)^{-1}(\mathbf{I} - \hat{\mathbf{z}}\hat{\mathbf{z}})$ . Substituting these two expressions to Eq. (S105) and solving them with respect to  $a$  and  $b$  yield

$$\varepsilon_I = \varepsilon_{BG}^{(2D)} (\mathbf{I} - \hat{\mathbf{z}}\hat{\mathbf{z}}) + \langle \varepsilon \rangle \hat{\mathbf{z}}\hat{\mathbf{z}}, \quad (\text{S108})$$

where  $\varepsilon_{BG}^{(2D)}$  is the Bruggeman approximation (also known as Self-Consistent Approximation or Coherent Potential Approximation) for 2D two-phase media [1, 19]:

$$\varepsilon_{BG}^{(2D)} = \frac{1}{2} \left[ 2 \langle \varepsilon \rangle - (\varepsilon_1 + \varepsilon_2) \pm \sqrt{[2 \langle \varepsilon \rangle - (\varepsilon_1 + \varepsilon_2)]^2 + 4 \varepsilon_1 \varepsilon_2} \right]. \quad (\text{S109})$$

We use Eq. (S109) with the “+” sign. Similar to what we did for Eq. (S107), we apply such a renormalization to the strong-contrast approximations [Eq. (S78) and Eq. (S79) at the three-point level] for obtaining the scaled strong-contrast approximations for transversely isotropic media:

$$\frac{\phi_p^2 [2\varepsilon_q \beta_{pq}^{(2D)}]^2}{2\varepsilon_q} \frac{\varepsilon_e^{TE}(k_q) + \varepsilon_q}{\varepsilon_e^{TE}(k_q) - \varepsilon_q} = \phi_p [2\varepsilon_q \beta_{pq}^{(2D)}] - A_2^{TE}(k_*^{TE}; \varepsilon_{BG}^{(2D)}) [2\varepsilon_q \beta_{pq}^{(2D)}]^2 - A_3^{TE}(k_*^{TE}; \varepsilon_{BG}^{(2D)}) [2\varepsilon_q \beta_{pq}^{(2D)}]^3, \quad (\text{S110})$$

$$\begin{aligned} \frac{[\phi_p (\varepsilon_p + \varepsilon_q) \beta_{pq}^{(2D)}]^2}{\varepsilon_e^{TM}(k_q) - \varepsilon_q} &= \phi_p [(\varepsilon_p + \varepsilon_q) \beta_{pq}^{(2D)}] - A_2^{TM}(k_*^{TM}; \langle \varepsilon \rangle) [(\varepsilon_p + \varepsilon_q) \beta_{pq}^{(2D)}]^2 \\ &\quad - A_3^{TM}(k_*^{TM}; \langle \varepsilon \rangle) [(\varepsilon_p + \varepsilon_q) \beta_{pq}^{(2D)}]^3, \end{aligned} \quad (\text{S111})$$

200 where  $k_*^{TE} \equiv k_q \sqrt{\varepsilon_{BG}^{(2D)} / \varepsilon_q}$  and  $k_*^{TM} \equiv k_q \sqrt{\langle \varepsilon \rangle / \varepsilon_q}$  are wave numbers in the optimal reference  
201 phase for TE and TM polarizations, respectively.

## 202 5. COMPARISON OF STRONG- AND WEAK-CONTRAST EXPANSIONS

203 Here, we analytically demonstrate how the linear fractional form of the strong-contrast expansion  
204 leads to lower-order truncations that accurately estimate the effective dielectric constant tensor  
205  $\varepsilon_e(\mathbf{k}_q, \omega)$ , even for large contrast ratios, compared to the standard perturbation expansions  
206 of  $\varepsilon_e(\mathbf{k}_q, \omega)$ , which we call *weak-contrast* expansions, which do not converge rapidly for large  
207 contrast ratios. For simplicity, we henceforth focus on the scaled strong-contrast expansion for the  
208 transverse polarization in layered media; see its third-order truncation in Eq. (S107). The reader  
209 can find an analogous discussion concerning strong-contrast and weak-contrast convergence  
210 properties of 3D statistically isotropic media in Ref. [4].

We first clarify how the strong-contrast expansion is formally different from its weak-contrast counterpart. As shown in Eq. (S45), the exact “strong-contrast expansion” is a rational function (or linear fractional form) of the effective dielectric constant  $\varepsilon_e^\perp(k_q)$ :

$$\frac{(\phi_p \varepsilon_q \delta)^2}{\varepsilon_e^\perp(k_q) - \varepsilon_q} = \phi_p \varepsilon_q \delta - \sum_{m=2}^{\infty} \delta^m A_m, \quad (\text{S112})$$

where  $\delta \equiv \varepsilon_p / \varepsilon_q - 1$ ,  $A_m = \varepsilon_q^m A_m^\perp(k_*, \langle \varepsilon \rangle)$  for  $m \geq 2$  and  $k_* \equiv k_q \sqrt{\langle \varepsilon \rangle / \varepsilon_q}$ . Thus, solving for  $\varepsilon_e^\perp(k_q)$  from the exact strong-contrast expansion [Eq. (S112)] yields the following rational function:

$$\frac{\varepsilon_e^\perp(k_q)}{\varepsilon_q} = 1 + \frac{\phi_p^2 (\varepsilon_q \delta)^2}{\phi_p \varepsilon_q \delta - \sum_{m=2}^{\infty} \delta^m A_m}, \quad (\text{S113})$$

On the other hand, the exact “weak-contrast expansion” of  $\varepsilon_e^\perp(k_q)$  is a power series of  $\varepsilon_e^\perp(k_q)$  itself around  $\delta = 0$ , i.e.,

$$\frac{\varepsilon_e^\perp(k_q)}{\varepsilon_q} = 1 + \sum_{m=1}^{\infty} \delta^m B_m, \quad (\text{S114})$$

where  $B_m$  is the wave-number-dependent coefficient accounting for the multiple-scattering effects at the  $m$ th order. Since Eq. (S113) and the exact weak-contrast series [Eq. (S114)] are identical as long as they are convergent, the  $m$ th-order term  $A_m$  can be related to  $B_m$ , i.e., the multiple scattering effects at the  $m$ th order. Specifically, the first four coefficients  $B_1, \dots, B_4$  are explicitly given in terms of  $A_m$  as

$$\begin{aligned} B_1 &= \phi_p \varepsilon_q \\ B_2 &= A_2 \\ B_3 &= [(A_2)^2 + A_3 \varepsilon_q \phi_p] / (\varepsilon_q \phi_p) \\ B_4 &= [(A_2)^3 + 2A_2 A_3 \varepsilon_q \phi_p + A_4 \varepsilon_q \phi_p^2] / \varepsilon_q \phi_p^2. \end{aligned}$$

Now, we show how the low-order truncation of the strong-contrast expansion accurately approximates the multiple-scattering effects through all orders. For simplicity, we explicitly write the 2nd-order truncation of the strong-contrast expansion from Eq. (S113):

$$\begin{aligned} \frac{\varepsilon_e^\perp(k_q)}{\varepsilon_q} &\approx 1 + \frac{\phi_p^2 x^2}{\phi_p x - x^2 A_2} \\ &= 1 + \phi_p x + A_2 x^2 + \frac{[A_2^2]}{\phi_p} x^3 + \frac{[A_2^3]}{\phi_p^2} x^4 + \dots \end{aligned} \quad (\text{S115})$$

Thus, comparing Eq. (S115) to Eq. (S114), we see that the second-order truncation of the strong-contrast expansion accurately approximates the  $m$ th-order term  $B_m$ , which accounts for the multiple scattering effects, of the exact weak-contrast expansion [Eq. (S114)] through all orders in terms of the second-order term  $A_2$ . The second-order truncation, Eq. (S115), can be thought of as an approximate but accurate resummed representation of the exact expansion [Eq. (S114)].

## 6. SIMULATION DETAILS

Here, we provide additional details about simulation procedures. We list simulation parameters for generating microstructures in Sec. A. We then provide details of FDTD simulations in Sec. B. In Sec. C, we describe the algorithm for extracting the effective dielectric constants.

### A. Generation of Model Microstructures

We numerically generate two models of 1D and 2D disordered hyperuniform media that enable us to generate layered and transversely isotropic media, respectively: nonstealthy hyperuniform (NSHU) polydisperse sphere packing in a matrix and stealthy hyperuniform (SHU) sphere packing in a matrix (see section 5 of the main text). For each model, we generate  $N_c$  different microstructures of  $N$  particles in a hypercubic periodic fundamental cell of side length  $L$  at unit number density  $\rho (\equiv N/L^d) = 1$ . We summarize all parameters in Table S1.

**Table S1.** Simulation parameters to generate the two disordered hyperuniform models for  $d = 1$  and 2: NSHU and SHU models. For each model,  $N_c$  is the number of distinct microstructures,  $L$  is the side length of the simulation box,  $\rho$  is the number density,  $N$  is the particle number,  $\phi_2$  is the packing fraction, and  $\rho^{1/d}a$  is particle radius. Specifically,  $N_c: \tilde{\chi}_v(k)$  is the number of microstructures used for computing the spectral density, and  $N_c: \text{FDTD}$  is the number of microstructures employed in the FDTD simulations. For SHU media, we list  $\chi$  values and exclusion diameter  $\sigma$  of soft-core interaction. For NSHU media,  $a$  stands for the mean particle radius, i.e.,  $a \equiv [\phi_2 / v_1(1)]^{1/d}$ .

| Model \ Parameters | $N_c: \tilde{\chi}_v(k)$ | $N_c: \text{FDTD}$ | $L$  | $\rho$ | $N$ | $\phi_2$ | $\rho^{1/d}a$ | $\sigma$ | $\chi$ |
|--------------------|--------------------------|--------------------|------|--------|-----|----------|---------------|----------|--------|
| 1D SHU             | 10000                    | 400                | 50.0 | 1.0    | 50  | 0.20     | 0.10          | 0.25     | 0.30   |
| 2D SHU             | 5000                     | 50                 | 10.0 | 1.0    | 100 | 0.25     | 0.2821        | 0.57     | 0.30   |
| 1D NSHU            | 10000                    | 400                | 50.0 | 1.0    | 50  | 0.20     | 0.10          | -        | -      |
| 2D NSHU            | 3000                     | 50                 | 10.0 | 1.0    | 100 | 0.25     | 0.2821        | -        | -      |

We generate 1D and 2D NSHU media as follows: In one dimension, we generate them by using the tessellation-based procedure [20, 21] from 1D equilibrium packings of packing fraction 0.20. Specifically, one begins with the Voronoi tessellation [1] of these progenitor point patterns. We then move the particle center in a Voronoi cell to its centroid and rescale the particle so that the packing fraction inside it is identical to a prescribed value  $\phi_2 < 1$ . The same process is repeated over all cells. The final packing fraction is  $\phi_2 = \sum_{j=1}^N v_1(a_j) / L^d = \rho v_1(a)$ , where  $\rho$  is the number density of particle centers and  $a$  represents the mean sphere radius. For  $d = 2$ , we apply the analogous procedure to 2D equilibrium packings of 0.30. The generated configurations are used to compute the spectral density and perform FDTD simulations.

We generate 1D and 2D SHU media by employing the revised collective-coordinate optimization technique described in section 5.B of the main text. This technique requires two additional parameters:  $\chi$  and  $\sigma$ . We set the  $\chi$  parameter, which is the ratio of constrained degrees  $\mathcal{M}$  of freedom to total number of degrees of freedom [22, 23] (i.e.,  $\chi \equiv \mathcal{M} / [d(N - 1)]$ ) to be  $\chi = 0.30$  for  $d = 1, 2$ . We choose the exclusion diameter  $\sigma$  of the soft-core repulsive potential to be  $\sigma = 0.25, 0.57$  for  $d = 1, 2$ , respectively. These configurations are used to compute spectral density and perform FDTD simulations.

## B. Finite-Difference Time-Domain (FDTD) Simulations

**Table S2.** Length parameters of FDTD simulations depicted in Fig. S2. We define  $\rho^{-1}$  and  $\rho^{-1/2}$  to be the length units for layered and transversely isotropic media, respectively.

| Parameters      | Layered Media ( $d = 1$ )              | Transversely Isotropic Media ( $d = 2$ ) |
|-----------------|----------------------------------------|------------------------------------------|
| L               | 50.0                                   | 10.0                                     |
| tpml            | $(0.05)^{-1}$ (the longest wavelength) |                                          |
| dpml            | 0.50                                   | 0.50                                     |
| dsrc            | 3.00                                   | 3.00                                     |
| ddet            | 3.00                                   | 3.00                                     |
| ddet2           | 1.50                                   | 1.50                                     |
| $\Delta$        | 0.50                                   | 0.50                                     |
| grid resolution | 80 pixels                              | 60 pixels                                |

We numerically verify the accuracy of our second-order formulas [Eq. (S107) and Eq. (S111) where  $A_3 = 0$ ] by showing excellent agreement with the effective dielectric constant found from simulations. For this purpose, we primarily perform the finite-difference time-domain (FDTD) [24] via an open-source FDTD package MEEP [25]. Figure S2 shows the FDTD simulation

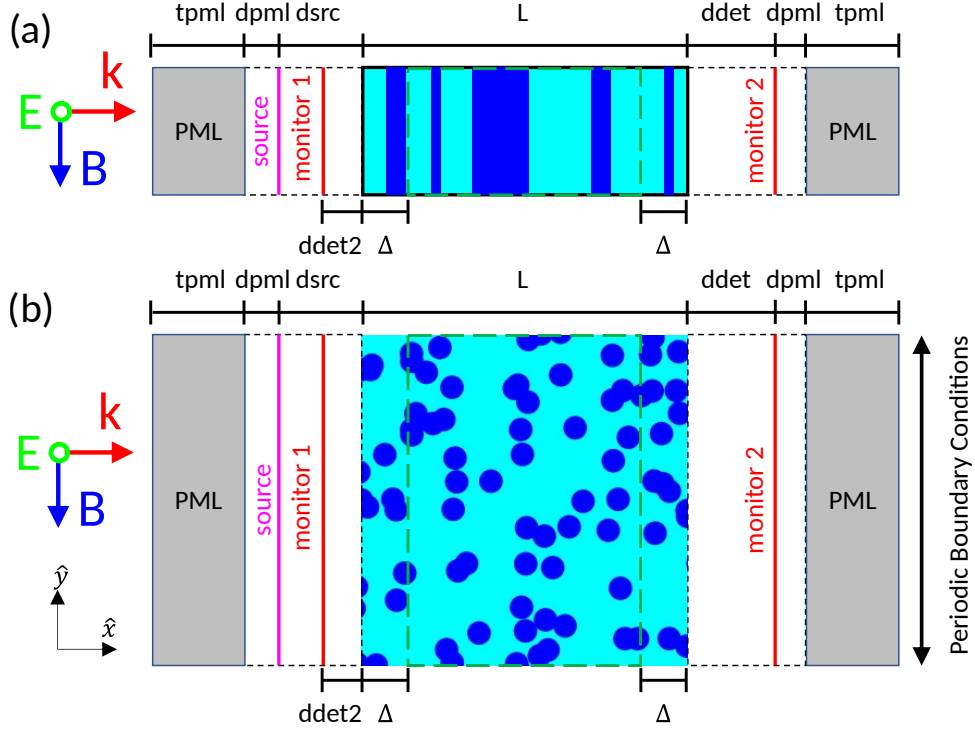

**Fig. S2.** Schematic of FDTD simulation setup for (a) layered and (b) transversely isotropic media. A Gaussian pulse of the electric field generated from the source plane (shown in the magenta line) is incident to the two-phase media of length  $L$ . The polarization of the pulse is transverse in (a) and TM in (b). We place the perfectly matched layers (PML, shown in the gray boxes) of thickness  $tpml$  at both ends of the simulation box to simulate the open boundary condition. For (b), we apply periodic boundary conditions along the  $y$  direction. In the homogenization procedure, we consider the fields in the region surrounded by a green dashed line.

248 setup. This figure shows the reference phase in white, and its dielectric constant is identical to  
 249  $\epsilon_1 = 1$ . The matrix and particle phases of the two-phase media are shown in cyan and dark blue,  
 250 respectively, and their dielectric constants are  $\epsilon_1 = 1, \epsilon_2 = 4$ , respectively. The specific values of  
 251 the lengths defined in Fig. S2 are listed in Table S2. Unlike the assumptions in the Sec. 2C and 3C,  
 252 we set the wave to propagate along the  $x$  axis to perform 1D simulations for layered media and  
 253 2D simulations for transversely isotropic media.

254 For each model of layered media, we perform simulations for 400 distinct configurations.  
 255 The source plane generates a planar Gaussian pulse whose wave number spectrum spans from  
 256  $k_1/\rho = 0.05$  to 4.05. Each simulation lasts until the mean electric field at monitor 2, shown in Fig.  
 257 S2(a), decays down to  $10^{-7}$  of its maximum value. After the dynamics simulation, we perform  
 258 temporal Fourier transformation to obtain electric field  $E_y(x; \omega)$ , dielectric displacement field  
 259  $D_y(x; \omega)$  at a given set of frequencies  $\omega$ . We take these two types of fields inside the green dashed  
 260 regions in Fig. S2(a), which covers the entire composite excluding by a distance  $\Delta$  from both ends,  
 261 to reduce the surface effects. These fields are used to extract the effective dielectric constant, as  
 262 described in Sec. 6C.

263 For each model of transversely isotropic media, we perform simulations for 50 distinct configura-  
 264 tions. The source plane generates a planar Gaussian pulse whose wave number spectrum spans  
 265 from  $k_1/\rho^{1/2} = 0.05$  to 4.05. Each simulation lasts until the mean electric field at monitor 2, shown  
 266 in Fig. S2(b), decays down to  $10^{-6}$  of its maximum value. After the dynamics simulation, we  
 267 perform temporal Fourier transformation to obtain electric field  $E_z(x; \omega)$ , dielectric displacement  
 268 field  $D_z(x; \omega)$  at a given set of frequencies  $\omega$ . We take these two types of fields inside the green  
 269 dashed regions in Fig. S2(b), which covers the entire composite excluding by a distance  $\Delta$  from

270 both ends, to reduce the surface effects. These fields are used to extract the effective dielectric  
 271 constant, as described in Sec. S6C.

### 272 C. Effective Dielectric Constants

**Algorithm S1.** Algorithm to find the effective wave number  $k_e$  from ensemble averages of electric field  $\langle E(x) \rangle$  at a given frequency  $\omega$  or, equivalently,  $k_{\text{inc}} = \sqrt{\epsilon_1} \omega / c$ . We set  $\epsilon = 10^{-2}$  and  $x[0] = 0$ . Here,  $\lambda_e$  is the effective wavelength, and  $\epsilon_e(0) = \phi_1 \epsilon_1 + \phi_2 \epsilon_2$ .

---

```

1: Inputs: 1D arrays of length  $n$ ;  $\{ \langle E(x) \rangle, \langle D(x) \rangle, x, \text{ and } \Delta x \}$  and float variables  $\{ k_{\text{inc}} \text{ and } \epsilon_e(0) \}$ 
2: Initialize:  $k_e \leftarrow 0.0 + 0.0i$ ,  $k_{\text{guess}} \leftarrow \sqrt{\epsilon_e(0)} k_{\text{inc}}$ 
3:  $E \leftarrow \text{Re}[\langle E(x) \rangle]$ 
4:  $\text{idx}[] \leftarrow \{ i \mid E[i] == 0 \}$  ▷ Find zeros of the electric field
5:  $\text{len} \leftarrow \text{the length of } \text{idx}$ 
6: if  $\text{len} < 3$  then ▷ Sample is shorter than  $1.5\lambda_e$ 
7:    $\epsilon_e \leftarrow \text{Compute Eq. (S117) at } k_e = k_{\text{guess}}$ 
8:    $k_e \leftarrow \sqrt{\epsilon_e} k_{\text{inc}}$ 
9: else ▷ Sample is longer than  $1.5\lambda_e$ 
10:   $M \leftarrow n - 1$ 
11:   $E_{\text{normal}} \leftarrow \langle E(x) \rangle / \max |\langle E(x) \rangle|$ 
12:  if  $\min_j |E_{\text{normal}}[j]| < \epsilon$  then ▷ If attenuation is strong,
13:     $M \leftarrow \min_l \{ \text{idx}[l] \mid |E_{\text{normal}}[\text{idx}[l]]| < \epsilon \}$  ▷ field becomes too noisy beyond  $x = x[M]$ .
14:  else ▷ If attenuation is weak
15:     $M \leftarrow \max_j \{ \text{idx}[j] \}$ 
16:     $k_i[0] \leftarrow \min_{j=\text{idx}[\text{len}-4], \dots, M} \{ -\ln(|E_{\text{normal}}[j]|) / x[j] \}$ 
17:     $k_i[1] \leftarrow \max_{j=\text{idx}[\text{len}-4], \dots, M} \{ -\ln(|E_{\text{normal}}[j]|) / x[j] \}$ 
18:     $\lambda_{\text{max}} \leftarrow 2 \max_{j=0, \dots, M-1} \{ x[\text{idx}[j+1]] - x[\text{idx}[j]] \}$ 
19:     $\lambda_{\text{min}} \leftarrow 2 \min_{j=0, \dots, M-1} \{ x[\text{idx}[j+1]] - x[\text{idx}[j]] \}$ 
20:     $k_r[0] \leftarrow 2\pi / \lambda_{\text{max}}$ 
21:     $k_r[1] \leftarrow 2\pi / \lambda_{\text{min}}$ 
22:     $x_{\text{slice}} \leftarrow x[\text{idx}[0], \dots, M]$ 
23:     $E_{\text{slice}} \leftarrow E[\text{idx}[0], \dots, M]$ 
24:    Fit Eq. (S116) to  $x_{\text{slice}}$  and  $E_{\text{slice}}$  with the constraints  $k_r[0] \leq \text{Re}[k_e] \leq k_r[1]$  and  $k_i[0] \leq \text{Im}[k_e] \leq k_i[1]$ 
    return  $k_e$  ▷ Return the effective wave number

```

---

273 Here, we describe how we numerically extract the effective dynamic dielectric constant  $\epsilon_e(k_1)$   
 274 from the electric and dielectric displacement fields obtained after the FDTD simulations; see Sec.  
 275 S6B. This algorithm is a minor revision of the method introduced for estimating the effective  
 276 properties of 2D and 3D statistically isotropic media beyond the long-wavelength regime [4].  
 277 Recently, it was employed for extracting the effective dielectric constant of stealthy hyperuniform  
 278 layered media [15].

For each model, from the FDTD simulations described in Sec. S6B, we obtain the electric  $E(x; \omega)$  and dielectric displacement  $D(x; \omega)$  fields for all configurations and frequencies. Using them, we compute their ensemble averages,  $\langle E(x; \omega) \rangle$  and  $\langle D(x; \omega) \rangle$ , at a given frequency  $\omega = ck_1 / \sqrt{\epsilon_1}$ . We then estimate the *effective wave number*  $k_e$  by fitting  $\text{Re}[\langle E(x; \omega) \rangle]$  with an exponentially decaying sinusoidal function (see Algorithm S1 for details):

$$y = A \exp(-\text{Im}[k_e]x) \cos(\text{Re}[k_e]x + \eta). \quad (\text{S116})$$

We compute the Fourier transforms  $\langle \tilde{D}(k_e, \omega) \rangle$  and  $\langle \tilde{E}(k_e, \omega) \rangle$  at  $k_e$  using the following relation:

$$\langle \tilde{f}(k_e; \omega) \rangle \equiv \int_{-L/2+\Delta}^{L/2-\Delta} \langle f(x; \omega) \rangle \exp(-ik_e x) dx.$$

Using these Fourier components, we finally obtain the effective dielectric constant  $\epsilon_e(k_1)$ :

$$\epsilon_e(k_1) = \langle \tilde{D}(k_e, \omega) \rangle / \langle \tilde{E}(k_e, \omega) \rangle. \quad (\text{S117})$$

## 7. ADDITIONAL RESULTS FROM FDTD SIMULATIONS

Here, we present an additional plot of the effective dielectric constants from FDTD simulations for layered media and transversely isotropic media generated from the NSHU model. For layered media with  $\phi_2 = 0.20$  and the contrast ratio  $\varepsilon_2/\varepsilon_1 = 4.0$ , we compare the scaled second-order formula [Eq. (S107) with  $A_3^\perp = 0$ ] to the FDTD simulation results; see Fig. S3 (a). For transversely isotropic media, we made an analogous comparison with  $\phi_2 = 0.25$  and contrast ratio  $\varepsilon_2/\varepsilon_1 = 4.0$ ; see Fig. S3(b). For both plots, the real and imaginary parts of these predictions show excellent agreement with the results from FDTD simulations up to  $k_1\rho^{-1/d} \lesssim 1.5$ , which is well beyond the long-wavelength regime. For small wave numbers, the imaginary parts are very small but not equal to zero.

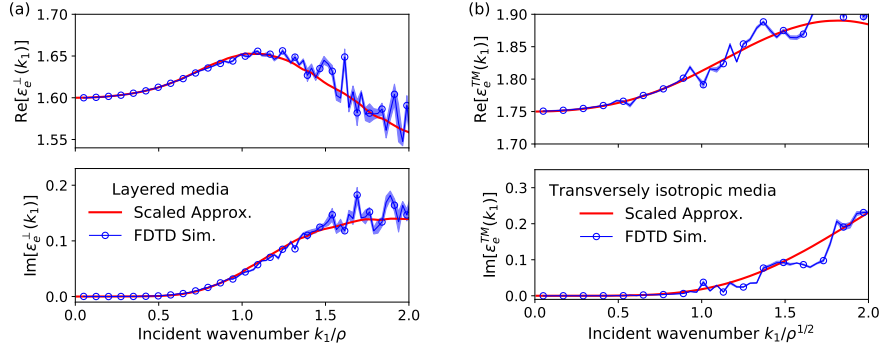

**Fig. S3.** Comparison of the predictions of the second-order strong-contrast approximations for the effective dynamic dielectric constant as a function of the dimensionless wave number for the NSHU model of  $\varepsilon_2/\varepsilon_1 = 4$  with various symmetries to FDTD simulations. We consider (a) layered media with  $\phi_2 = 0.20$  and (b) transversely isotropic media with  $\phi_2 = 0.25$ . Values of approximations in (a) and (b) are computed from Eq. (S107) and Eq. (S111) with  $A_3(k) = 0$ , respectively.

## 8. KRAMERS-KRONIG RELATIONS

Here, we show that the second-order strong-contrast approximations [Eq. (S107) and Eq. (S111)] satisfy the Kramers-Kronig relations [26, 27]

$$\text{Re}[\varepsilon_e(k_q)] = \varepsilon_\infty + \frac{2}{\pi} \text{p.v.} \int_0^\infty dq \frac{q \text{Im}[\varepsilon_e(q)]}{q^2 - k_q^2}, \quad (\text{S118})$$

$$\text{Im}[\varepsilon_e(k_q)] = -\frac{2k_q}{\pi} \text{p.v.} \int_0^\infty dq \frac{\text{Re}[\varepsilon_e(q)] - \varepsilon_\infty}{q^2 - k_q^2}, \quad (\text{S119})$$

where p.v. stands for the Cauchy principal value of the integral, and  $\varepsilon_\infty \equiv \lim_{k_1 \rightarrow \infty} \varepsilon_e(k_1)$ . For this purpose, as discussed in Ref. [4, 26], it is sufficient to show that  $\varepsilon_e(k_q)$  meets the following three conditions:

- (i)  $\varepsilon_e(k_q)$  is an analytic function in the *upper half-plane* of  $k_q$ , in which  $\text{Im}[k_q] \geq 0$ ;
- (ii)  $\varepsilon_e(k_q) - \varepsilon_\infty$  vanishes faster than or equal to  $1/|k_q|$  as  $|k_q|$  goes to infinity; and
- (iii) The real and imaginary parts of  $\varepsilon_e(k_q) - \varepsilon_\infty$  are even and odd functions of  $k_q$ , respectively.

For layered media, we can immediately confirm the conditions (i) and (iii) from the formula for the nonlocal attenuation function [Eq. (S40)]. Furthermore, Eq. (S38) yields the large- $k$  asymptotic behaviors of  $F^{(1D)}(k)$ :

$$F^{(1D)}(k) \sim \begin{cases} ic_1 k, & \text{typical nonhyperuniform media,} \\ -\frac{\phi_p(1-\phi_p)}{4} + ic_2/k, & \text{hyperuniform media} \end{cases}, \quad (k \rightarrow \infty) \quad (\text{S120})$$

where  $c_1$  and  $c_2$  are some positive constants. Therefore, we also confirm the condition (ii), i.e., Eq. (S107) converges to  $\varepsilon_\infty$  as fast as  $1/k_q$  for large  $k_q$ , where

$$\varepsilon_\infty \equiv \lim_{k_q \rightarrow \infty} \varepsilon_e^\perp(k_q) = \begin{cases} \varepsilon_q, & \text{typical nonhyperuniform media,} \\ \varepsilon_q \left[ \frac{4\varepsilon_q + \varepsilon_p \beta_{pq}^{(1D)}(1+3\phi_p)}{4\varepsilon_q + \varepsilon_p \beta_{pq}^{(1D)}(1-\phi_p)} \right], & \text{hyperuniform media} \end{cases}.$$

Thus, Eq. (S107) meets the Kramers-Kronig relations. One can easily confirm that the formula [Eq. (S111)] in transversely isotropic media also meets these three conditions from the properties of  $F^{(2D)}(k_q)$ , shown in Ref. [4]. Such predictions are reasonable because the requirements (i) and (ii) of the Kramers-Kronig relations come from the causality connections of a physical response [26], and the nonlocal attenuation functions  $F^{(1D)}(k)$  and  $F^{(2D)}(k)$  in those approximations involve the retarded Green's function given in Eq. (S4) that accounts for causality.

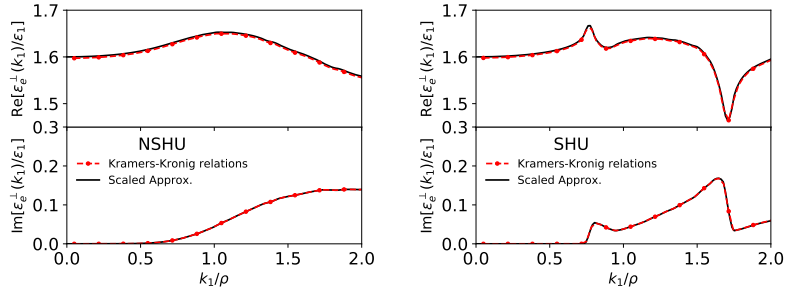

**Fig. S4.** Numerical verifications of the Kramers-Kronig relations for the second-order strong-contrast approximation for layered media [Eq. (S107), where  $A_3^\perp = 0$ ]. We consider two models of disordered hyperuniform layered media of  $\phi_2 = 0.2$  and contrast ratio  $\varepsilon_2/\varepsilon_1 = 4$ : (a) NSHU and (b) SHU models. In the upper panels, we compare the real part  $\text{Re}[\varepsilon_e(k_1)]$  of the approximation to that evaluated from the Kramers-Kronig relation Eq. (S118) and the imaginary part of the strong-contrast approximation. In the lower panels, we compare the imaginary part  $\text{Im}[\varepsilon_e(k_1)]$  of the approximation to that evaluated from Eq. (S119) and the real part of the approximation. The predictions from the approximation and its transform via Kramers-Kronig relations show excellent agreement.

For illustrative purposes, we compare the effective dielectric constant from the second-order approximations for layered [Eq. (S107), where  $A_3^\perp = 0$ ] and transversely isotropic [Eq. (S111), where  $A_3^{TM} = 0$ ] media to their transformation via the Kramers-Kronig relations; see Figs. S4 and S5, respectively. For both layered and transversely isotropic media, we consider the NSHU and SHU models; see Sec. 6A. Specifically, in the upper panels of Figs. S4 and S5, we present the predictions of  $\text{Re}[\varepsilon_e(k_1)]$  and those evaluated by using the Kramers-Kronig relation [Eq. (S118)] and  $\text{Im}[\varepsilon_e(k_1)]$  from the approximations. Similarly, in the lower panels, we compare  $\text{Im}[\varepsilon_e(k_1)]$  from the approximation with the calculation of Eq. (S119) by using  $\text{Re}[\varepsilon_e(k_1)]$  from the approximations. Computing the Kramers-Kronig relations, we carry out numerical integrals with an upper limit of  $q = 74/\rho$ . In both panels, the two scaled second-order formulas and their transformations via the Kramers-Kronig relations show excellent agreement, which numerically verifies that our approximations satisfy these relations.

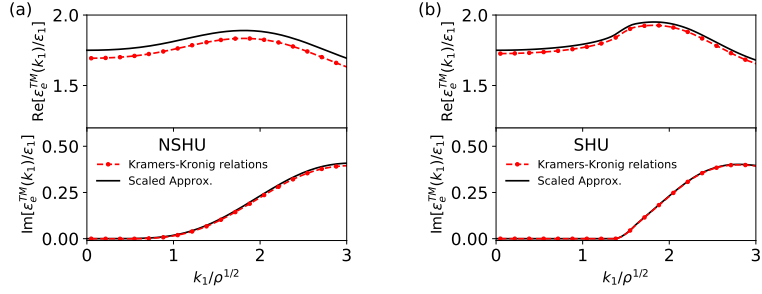

**Fig. S5.** Numerical verifications of the Kramers-Kronig relations for the second-order strong-contrast approximation for transversely isotropic media given in Eq. (S111), where  $A_3^{TM} = 0$ . We consider two models of disordered hyperuniform transversely isotropic media of  $\phi_2 = 0.25$  and contrast ratio  $\varepsilon_2/\varepsilon_1 = 4$ : (a) NSHU and (b) SHU models. In the upper panels, we compare the real part  $\text{Re}[\varepsilon_e(k_1)]$  of the approximation to that evaluated from the Kramers-Kronig relation Eq. (S118) and the imaginary part of the approximation. In the lower panels, we compare the imaginary part  $\text{Im}[\varepsilon_e(k_1)]$  of the approximation to that evaluated from Eq. (S119) and the real part of the approximation. The predictions from the approximation and its transform via Kramers-Kronig relations show excellent agreement.

## REFERENCES

1. S. Torquato, *Random Heterogeneous Materials: Microstructure and Macroscopic Properties*, no. 16 in *Interdisciplinary Applied Mathematics* (Springer Science & Business Media, New York, 2002).
2. S. Torquato and G. Stell, "Microstructure of two-phase random media. {I}. {T}he  $n$ -point probability functions," *J. Chem. Phys.* **77**, 2071–2077 (1982).
3. P. Debye, H. R. Anderson Jr, and H. Brumberger, "Scattering by an inhomogeneous solid. ii. the correlation function and its application," *J. Appl. Phys.* **28**, 679–683 (1957).
4. S. Torquato and J. Kim, "Nonlocal effective electromagnetic wave characteristics of composite media: Beyond the quasistatic regime," *Phys. Rev. X* **11**, 021002 (2021).
5. M. C. Rechtsman and S. Torquato, "Effective dielectric tensor for electromagnetic wave propagation in random media," *J. Appl. Phys.* **103**, 084901 (2008).
6. A. Yaghjian, "Electric dyadic green's functions in the source region," *Proc. IEEE* **68**, 248–263 (1980).
7. Y. A. Ryzhov, V. V. Tamoikin, and V. I. Tatarskii, "Spatial dispersion of inhomogeneous media," *Sov. Phys. JETP* **21**, 433 (1965).
8. L. Tsang and J. A. Kong, "Scattering of electromagnetic waves from random media with strong permittivity fluctuations," *Rádió Sci.* **16**, 303–320 (1981).
9. V. M. Agranovich and V. Ginzburg, *Crystal Optics with Spatial Dispersions, and Excitations*, Springer Series in Solid-State Sciences (Springer, Berlin, Heidelberg, 1984), 2nd ed.
10. A. V. Chebykin, A. A. Orlov, A. V. Vozianova, S. I. Maslovski, Yu. S. Kivshar, and P. A. Belov, "Nonlocal effective medium model for multilayered metal-dielectric metamaterials," *Phys. Rev. B* **84**, 115438 (2011).
11. U. Frisch, *Probabilistic Methods in Applied Mathematics*, vol. I and II (Academic Press, New York, 1968).
12. P. Sheng, *Introduction to wave scattering, localization, and mesoscopic phenomena*, no. 88 in Springer series in materials science (Springer, Berlin ; New York, 2006), 2nd ed.
13. A. Cazé and J. C. Schotland, "Diagrammatic and asymptotic approaches to the origins of radiative transport theory: tutorial," *J. Opt. Soc. Am. A* **32**, 1475 (2015).
14. K. Vynck, R. Pierrat, R. Carminati, L. S. Froufe-Pérez, F. Scheffold, R. Sapienza, S. Vignolini, and J. J. Sáenz, "Light in correlated disordered media," *ArXiv210613892 Cond-Mat Physicsphysics* (2021).
15. J. Kim and S. Torquato, "Effective electromagnetic wave properties of disordered stealthy hyperuniform layered media beyond the quasistatic regime," *Optica* **10**, 965 (2023).
16. J. Stewart, *Calculus: early transcendentals* (Cengage Learning, Boston, MA, USA, 2016), 8th ed.
17. G. Arfken, H. J. Weber, G. B. Arfken, and H.-J. Weber, *Mathematical methods for physicists* (Elsevier Academic Press, Amsterdam, Heidelberg, 2008), 6th ed.

- 350 18. T. G. Mackay, A. Lakhtakia, and W. S. Weiglhofer, "Strong-property-fluctuation theory for  
351 homogenization of bianisotropic composites: Formulation," *Phys. Rev. E* **62**, 6052–6064  
352 (2000).
- 353 19. D. A. G. Bruggeman, "Berechnung verschiedener physikalischer konstanten von heterogenen  
354 substanzen. i. dielektrizitätskonstanten und leitfähigkeiten der mischkörper aus isotropen  
355 substanzen," *Ann. der Physik* **416**, 636–664 (1935).
- 356 20. J. Kim and S. Torquato, "New tessellation-based procedure to design perfectly hyperuniform  
357 disordered dispersions for materials discovery," *Acta Mater.* **168**, 143–151 (2019).
- 358 21. J. Kim and S. Torquato, "Methodology to construct large realizations of perfectly hyperuni-  
359 form disordered packings," *Phys. Rev. E* **99**, 052141 (2019).
- 360 22. G. Zhang, F. Stillinger, and S. Torquato, "Ground states of stealthy hyperuniform potentials:  
361 I. entropically favored configurations," *Phys. Rev. E* **92**, 022119 (2015).
- 362 23. S. Torquato, G. Zhang, and F. H. Stillinger, "Ensemble theory for stealthy hyperuniform  
363 disordered ground states," *Phys. Rev. X* **5**, 021020 (2015).
- 364 24. A. Taflove, S. G. Johnson, and A. Oskooi, *Advances in FDTD Computational Electrodynamics:  
365 Photonics and Nanotechnology* (Artech House, Boston, 2013).
- 366 25. A. F. Oskooi, D. Roundy, M. Ibanescu, P. Bermel, J. D. Joannopoulos, and S. G. Johnson,  
367 "Meep: A flexible free-software package for electromagnetic simulations by the fdtd method,"  
368 *Comput. Phys. Commun.* **181**, 687–702 (2010).
- 369 26. J. D. Jackson, *Classical Electrodynamics* (John Wiley & Sons, Inc., New York, 1999), 3rd ed.
- 370 27. G. W. Milton, D. J. Eyre, and J. V. Mantese, "Finite frequency range kramers-kronig relations:  
371 Bounds on the dispersion," *Phys. Rev. Lett.* **79**, 3062–3065 (1997).
